# Supplementary material for: Using validated reanalysis data to investigate the impact of the PV system configurations at high penetration levels in European countries
Source: arXiv:1807.10044 source file (2018-07-26)
Supplement: Supplementary file 1 [file 20180710_Supplementary_materials_Using_validated_reanalysis_data.pdf]

# Supplementary materials for “Using validated reanalysis data to investigate the impact of the PV system configurations at high penetration levels in European countries”

Marta Victoria<sup>a,\*</sup>, Gorm B. Andresen<sup>a</sup>

<sup>a</sup>*Department of Engineering, Aarhus University, Inge Lehmanns Gade 10, 8000 Aarhus C, Denmark*

## 1. Preliminary analysis: reanalysis capability to capture local atmospheric effects

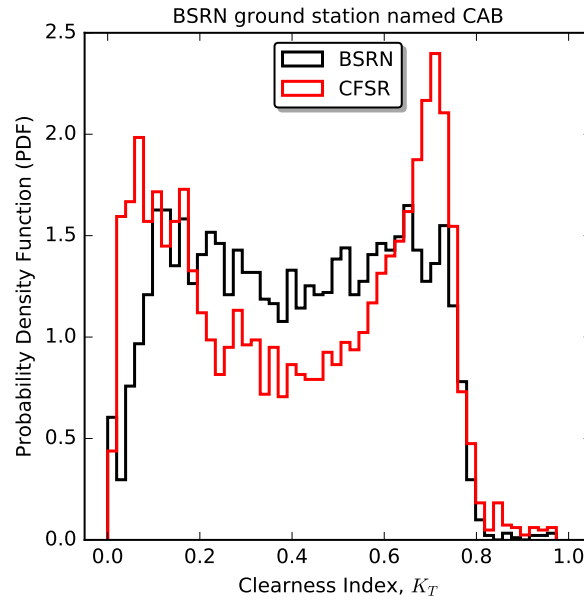

Figure 1: Probability Density Function (PDF) of the clearness index  $K_t$  calculated from measurements at the BSRN station named CAB and from the CFSR reanalysis dataset. The bin sizes are 0.02.

\*Corresponding author

Email address: [mvp@eng.au.dk](mailto:mvp@eng.au.dk) (Marta Victoria)

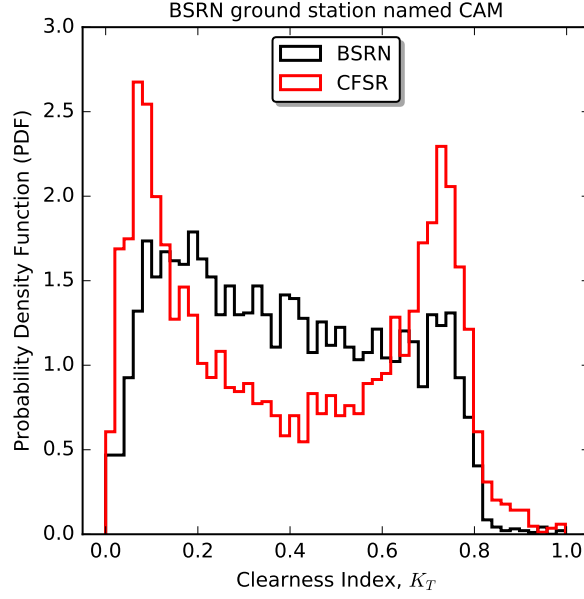

Figure 2: Probability Density Function (PDF) of the clearness index  $K_i$  calculated from measurements at the BSRN station named CAM and from the CFSR reanalysis dataset. The bin sizes are 0.02.

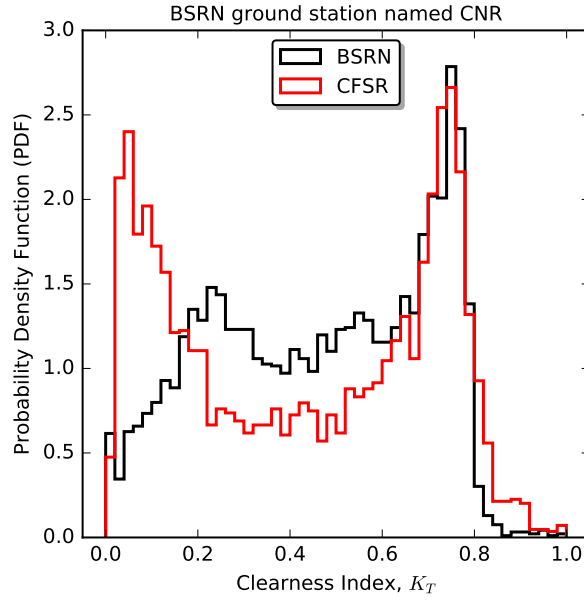

Figure 3: Probability Density Function (PDF) of the clearness index  $K_i$  calculated from measurements at the BSRN station named CNR and from the CFSR reanalysis dataset. The bin sizes are 0.02.

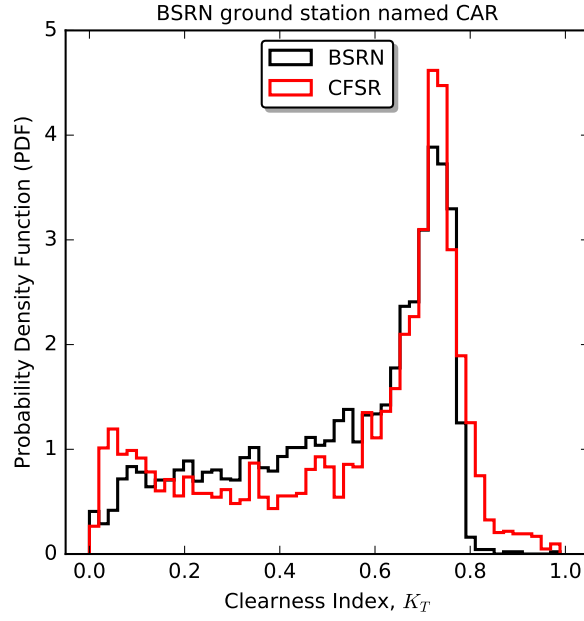

Figure 4: Probability Density Function (PDF) of the clearness index  $K_t$  calculated from measurements at the BSRN station named CAR and from the CFSR reanalysis dataset. The bin sizes are 0.02.

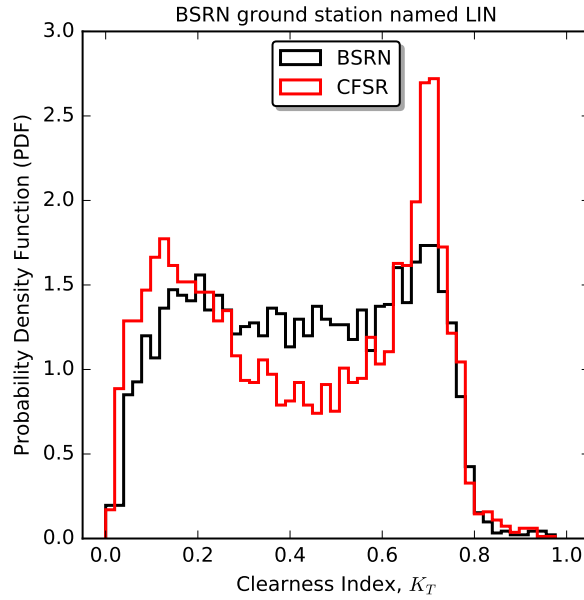

Figure 5: Probability Density Function (PDF) of the clearness index  $K_t$  calculated from measurements at the BSRN station named LIN and from the CFSR reanalysis dataset. The bin sizes are 0.02.

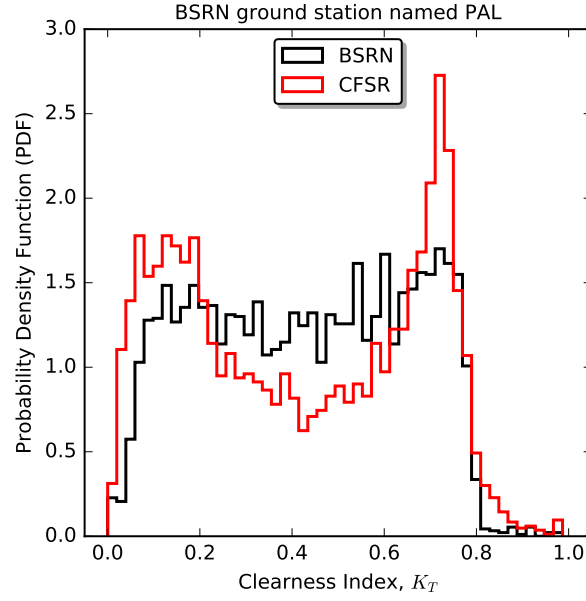

Figure 6: Probability Density Function (PDF) of the clearness index  $K_i$  calculated from measurements at the BSRN station named PAL and from the CFSR reanalysis dataset. The bin sizes are 0.02.

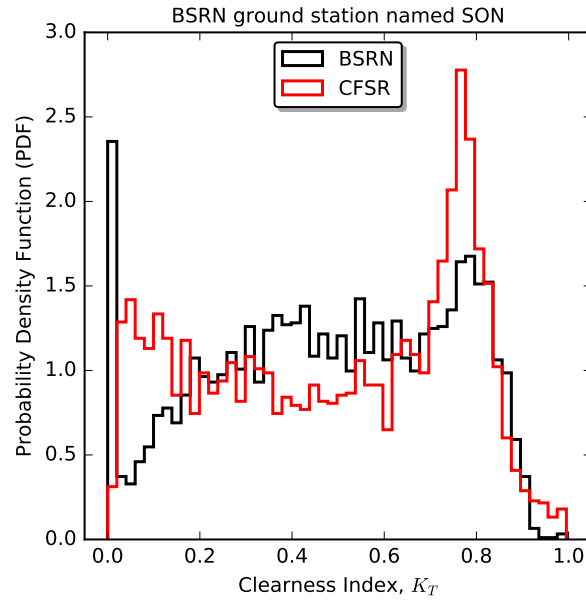

Figure 7: Probability Density Function (PDF) of the clearness index  $K_i$  calculated from measurements at the BSRN station named SON and from the CFSR reanalysis dataset. The bin sizes are 0.02.

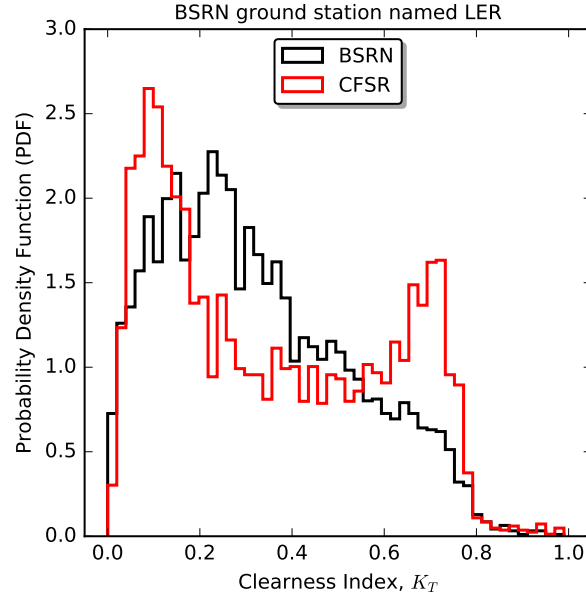

Figure 8: Probability Density Function (PDF) of the clearness index  $K_i$  calculated from measurements at the BSRN station named LER and from the CFSR reanalysis dataset. The bin sizes are 0.02.

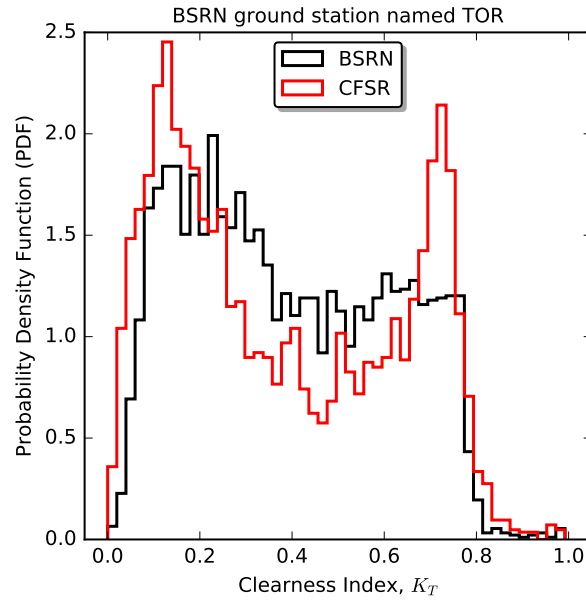

Figure 9: Probability Density Function (PDF) of the clearness index  $K_i$  calculated from measurements at the BSRN station named TOR and from the CFSR reanalysis dataset. The bin sizes are 0.02.

## 2. Monthly correction factors

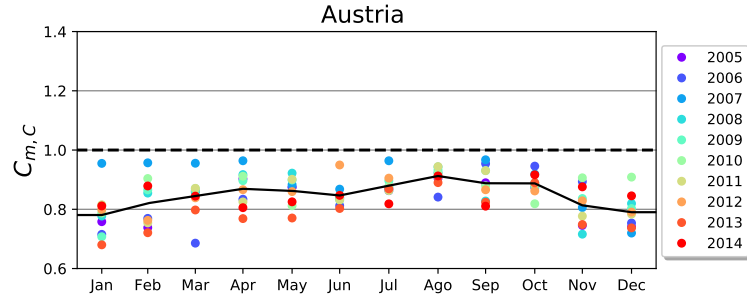

Figure 10: Monthly correction factors  $C_{m,s}$  for Austria .

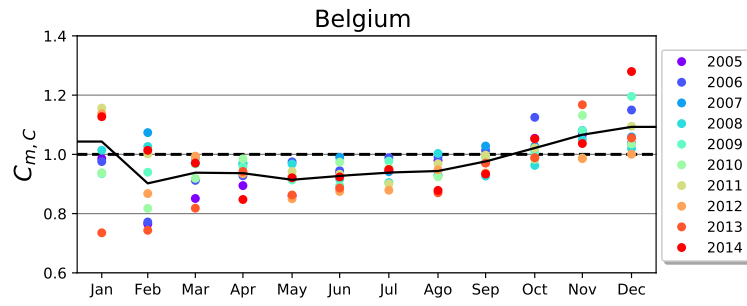

Figure 11: Monthly correction factors  $C_{m,s}$  for Belgium .

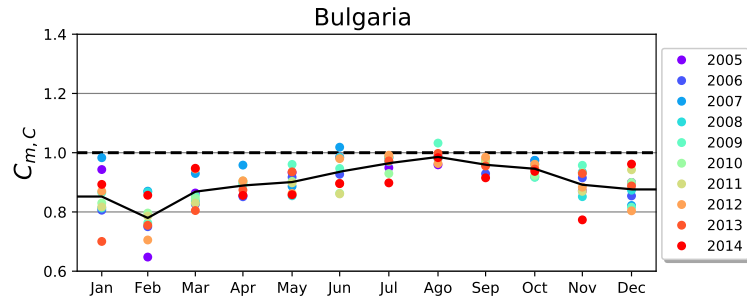

Figure 12: Monthly correction factors  $C_{m,s}$  for Bulgaria .

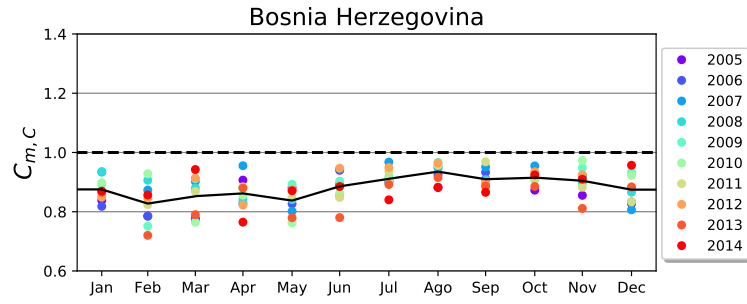

Figure 13: Monthly correction factors  $C_{m,s}$  for Bosnia Herzegovina.

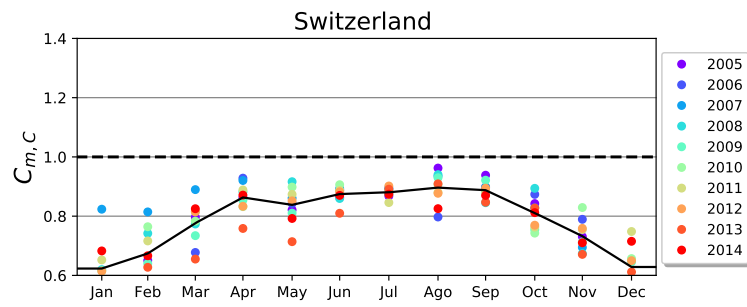

Figure 14: Monthly correction factors  $C_{m,s}$  for Switzerland .

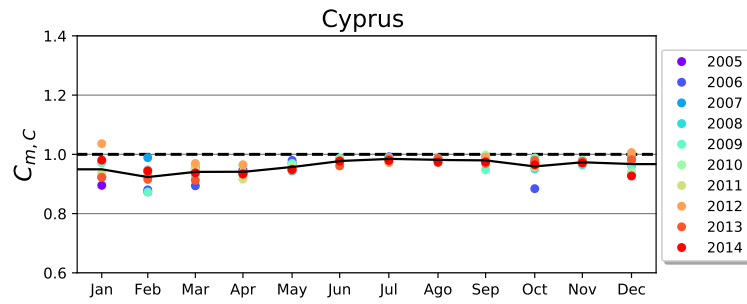

Figure 15: Monthly correction factors  $C_{m,s}$  for Cyprus .

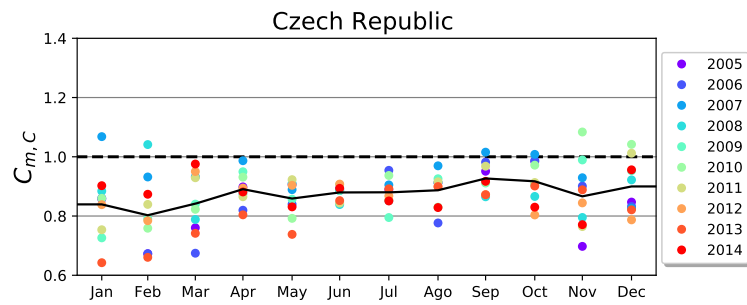

Figure 16: Monthly correction factors  $C_{m,s}$  for Czech Republic .

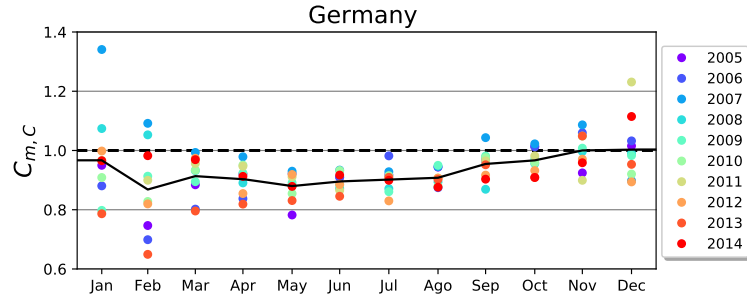

Figure 17: Monthly correction factors  $C_{m,s}$  for Germany .

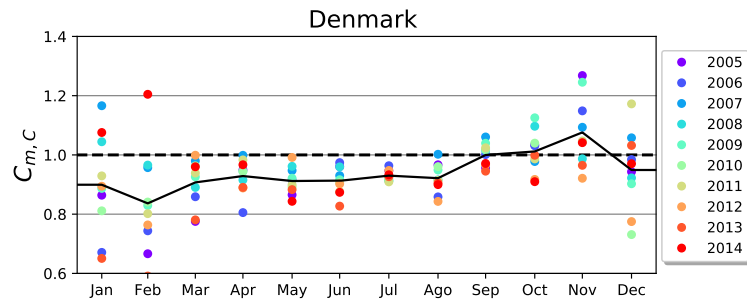

Figure 18: Monthly correction factors  $C_{m,s}$  for Denmark .

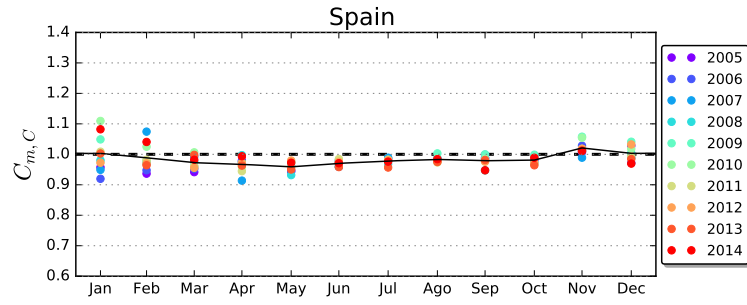

Figure 19: Monthly correction factors  $C_{m,s}$  for Spain .

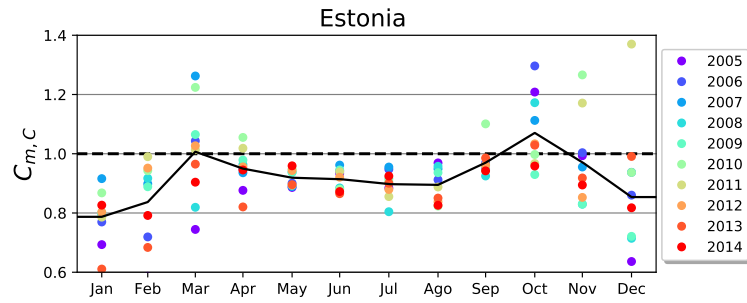

Figure 20: Monthly correction factors  $C_{m,s}$  for Estonia .



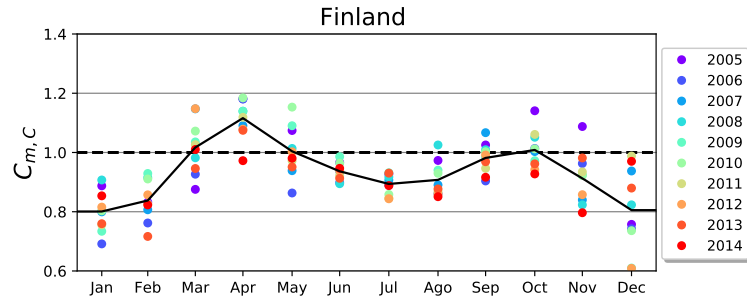

Figure 21: Monthly correction factors  $C_{m,s}$  for Finland .

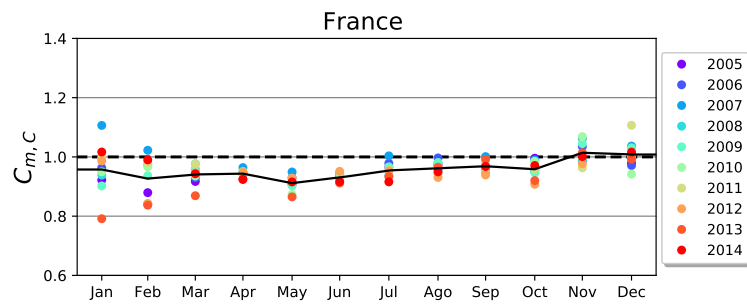

Figure 22: Monthly correction factors  $C_{m,s}$  for France .

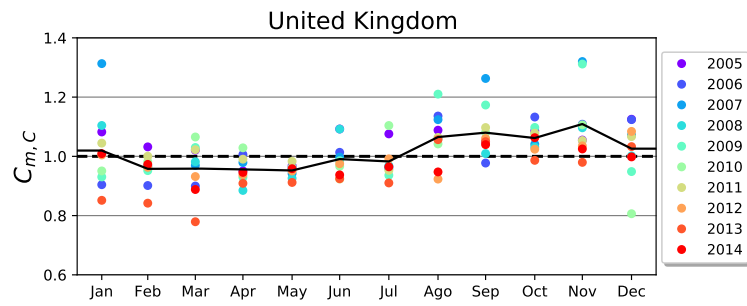

Figure 23: Monthly correction factors  $C_{m,s}$  for United Kingdom .

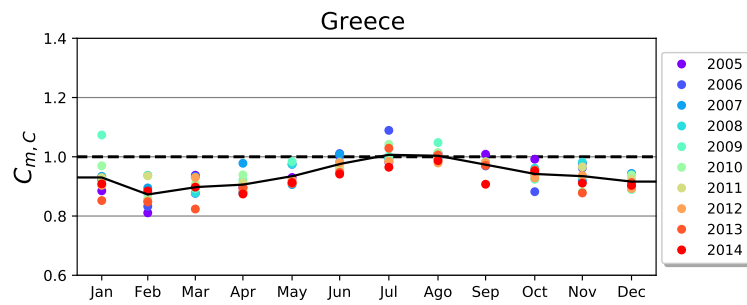

Figure 24: Monthly correction factors  $C_{m,s}$  for Greece .

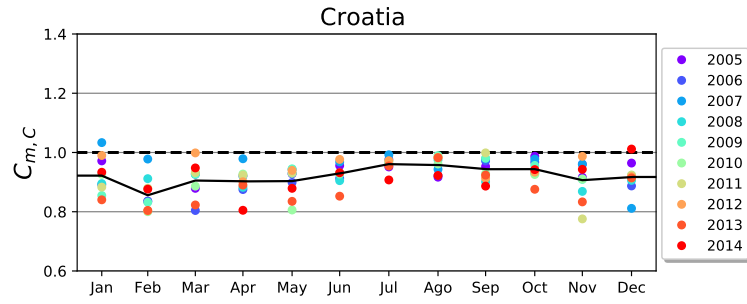

Figure 25: Monthly correction factors  $C_{m,s}$  for Croatia .

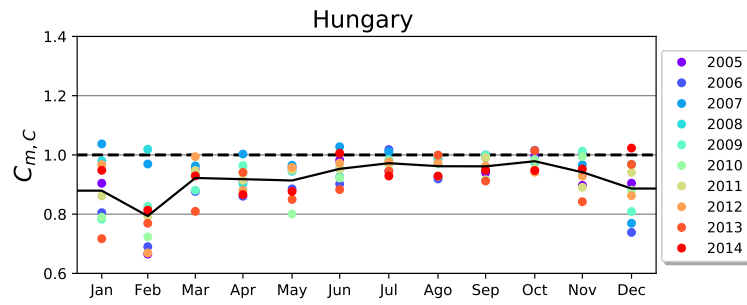

Figure 26: Monthly correction factors  $C_{m,s}$  for Hungary .

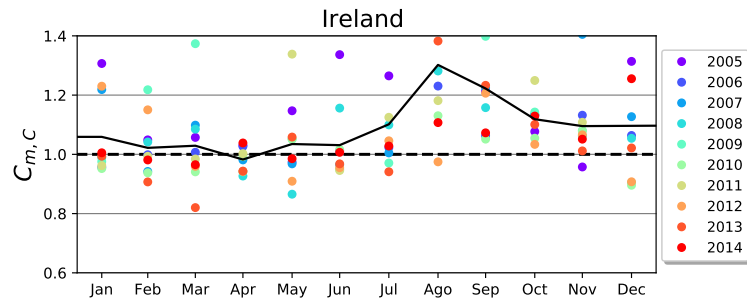

Figure 27: Monthly correction factors  $C_{m,s}$  for Ireland .

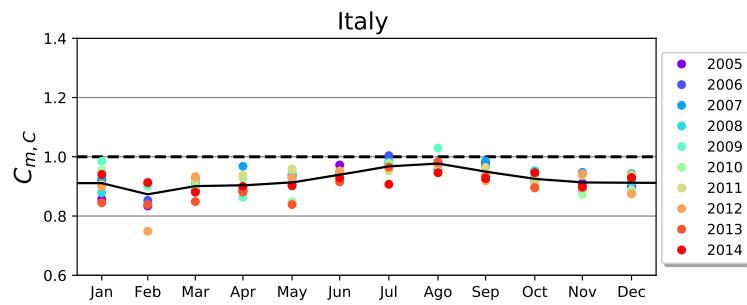

Figure 28: Monthly correction factors  $C_{m,s}$  for Italy .

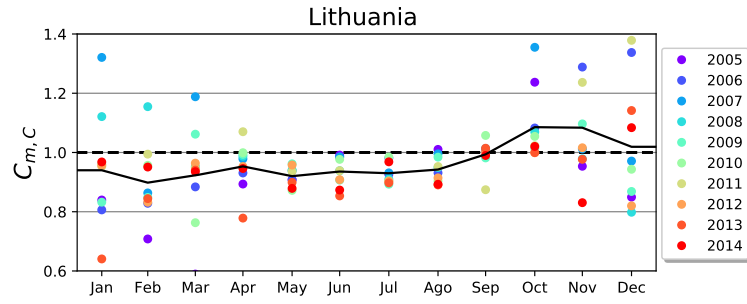

Figure 29: Monthly correction factors  $C_{m,s}$  for Lithuania .

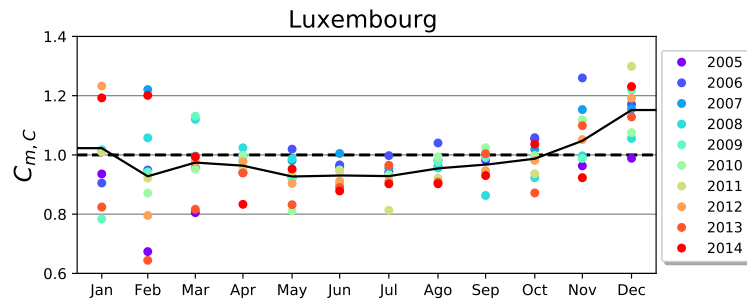

Figure 30: Monthly correction factors  $C_{m,s}$  for Luxembourg .

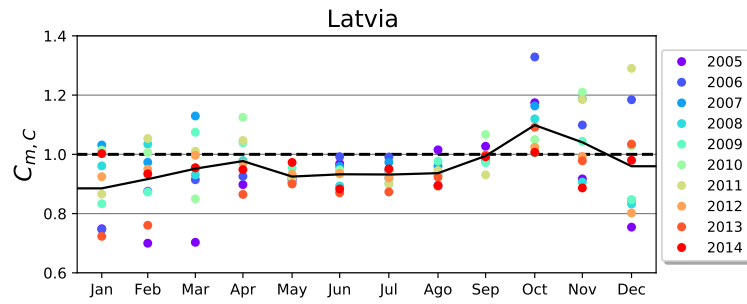

Figure 31: Monthly correction factors  $C_{m,s}$  for Latvia .

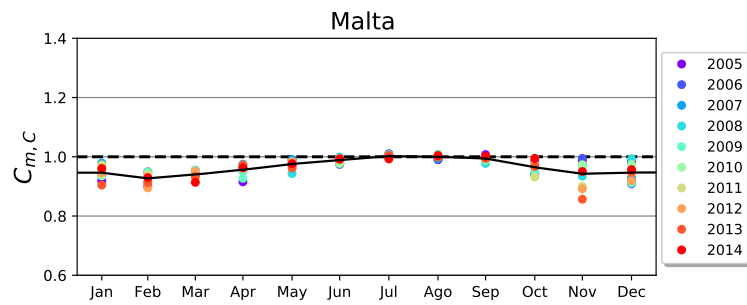

Figure 32: Monthly correction factors  $C_{m,s}$  for Malta .

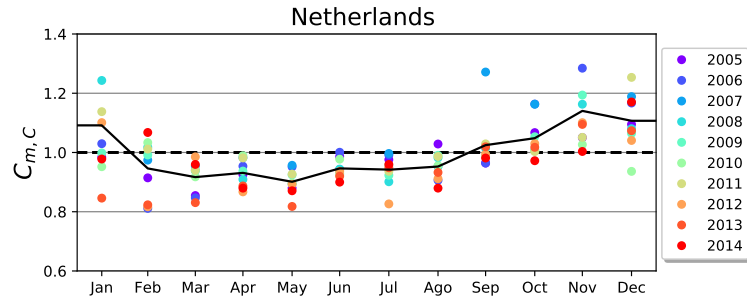

Figure 33: Monthly correction factors  $C_{m,s}$  for Netherlands .

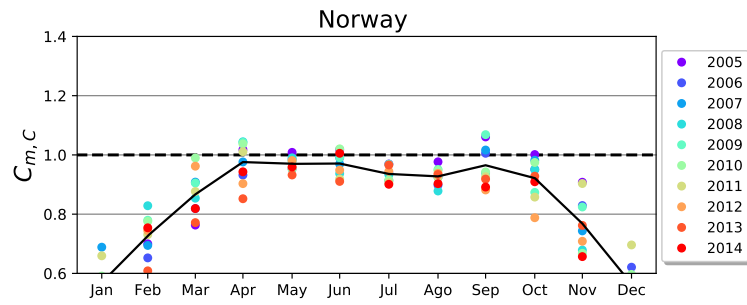

Figure 34: Monthly correction factors  $C_{m,s}$  for Norway .

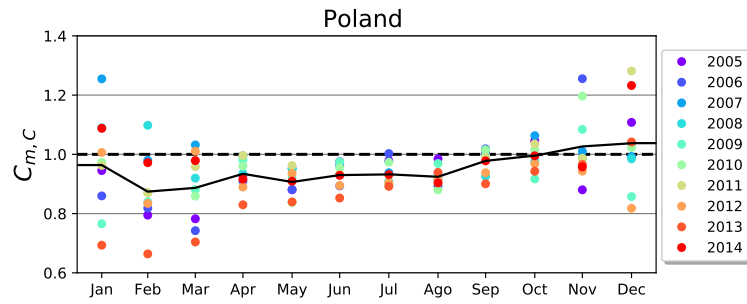

Figure 35: Monthly correction factors  $C_{m,s}$  for Poland .

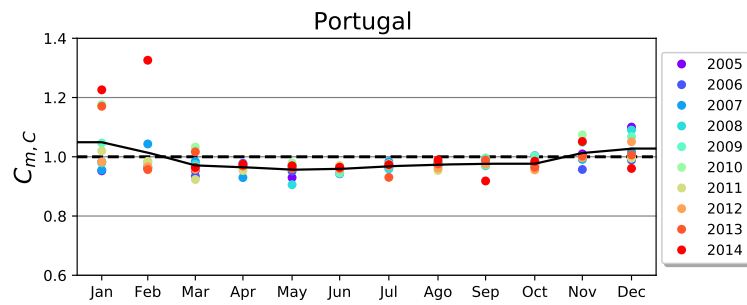

Figure 36: Monthly correction factors  $C_{m,s}$  for Portugal .

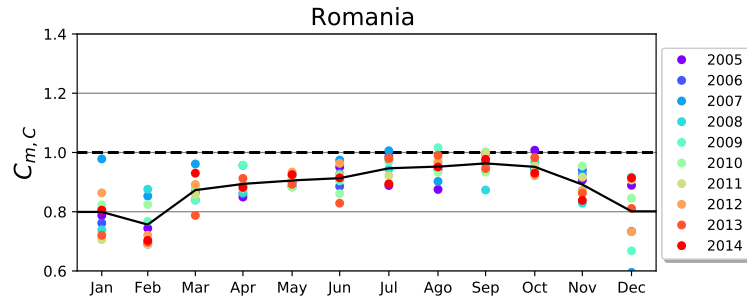

Figure 37: Monthly correction factors  $C_{m,s}$  for Romania .

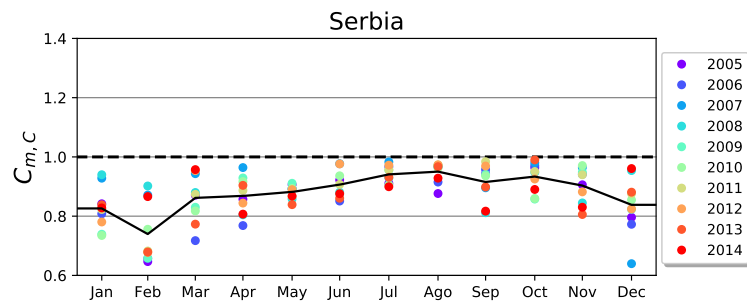

Figure 38: Monthly correction factors  $C_{m,s}$  for Serbia.

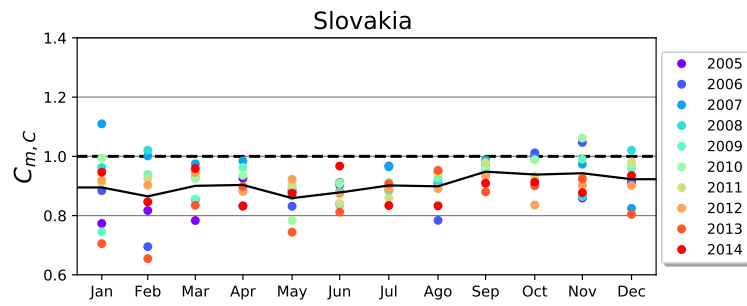

Figure 39: Monthly correction factors  $C_{m,s}$  for Slovakia .

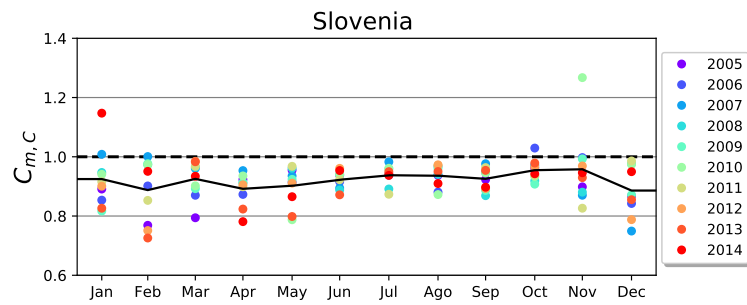

Figure 40: Monthly correction factors  $C_{m,s}$  for Slovenia .

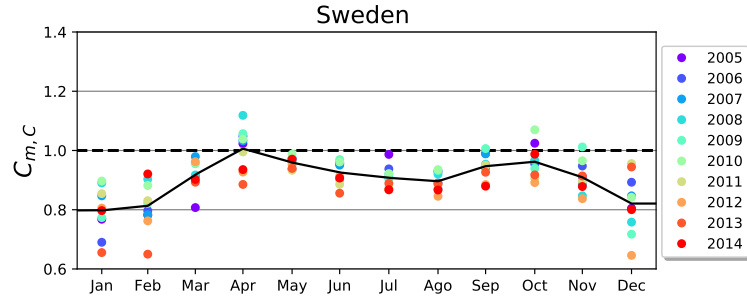

Figure 41: Monthly correction factors  $C_{m,s}$  for Sweden .

### 3. Maximum irradiance in days around solstice

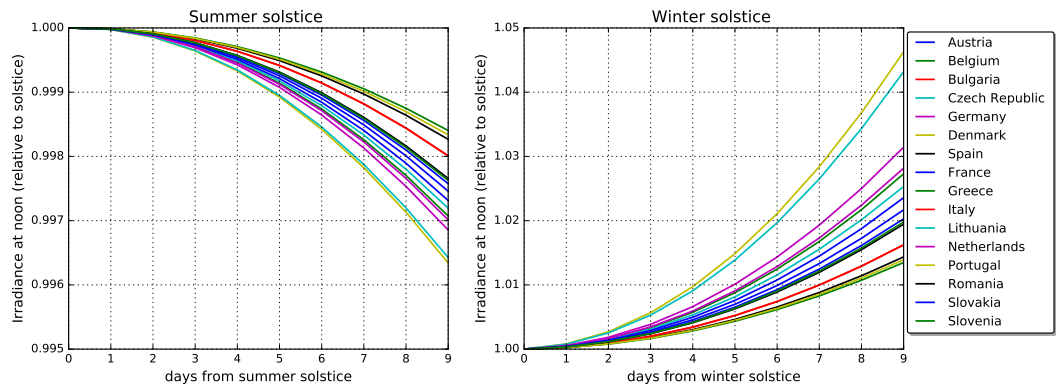

Figure 42: Evolution of maximum daily irradiance, relative to irradiance in the summer (left) and winter (right) solstices.

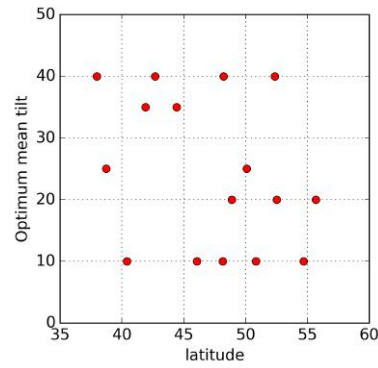

Figure 43: Mean of the best Gaussian distribution representing tilt angles in every country vs. latitude of the capital.

### 4. QQ plots with different time integration

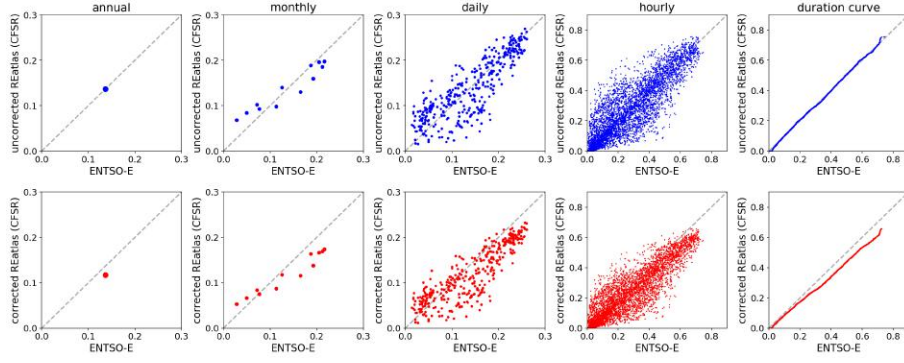

Figure 44: QQ plots comparing modeled and historical capacity factors for Austria integrated throughout four different time periods (from left to right: year, month, day, hour). The rightest column shows the QQ plot for the duration curve (sorted hourly capacity factors).

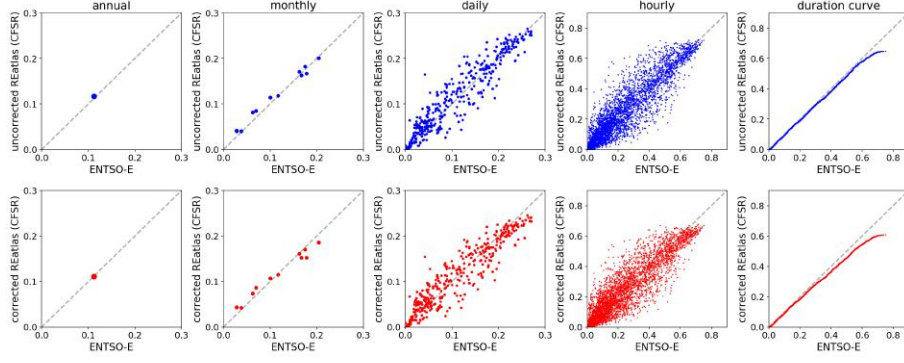

Figure 45: QQ plots comparing modeled and historical capacity factors for Belgium integrated throughout four different time periods (from left to right: year, month, day, hour). The rightest column shows the QQ plot for the duration curve (sorted hourly capacity factors).

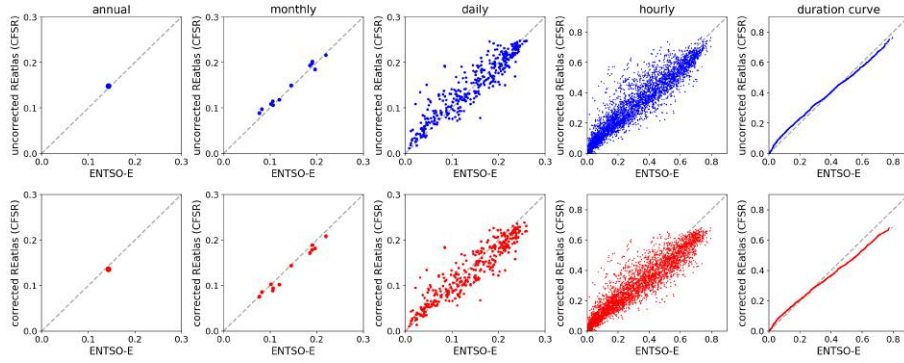

Figure 46: QQ plots comparing modeled and historical capacity factors for Bulgaria integrated throughout four different time periods (from left to right: year, month, day, hour). The rightest column shows the QQ plot for the duration curve (sorted hourly capacity factors).

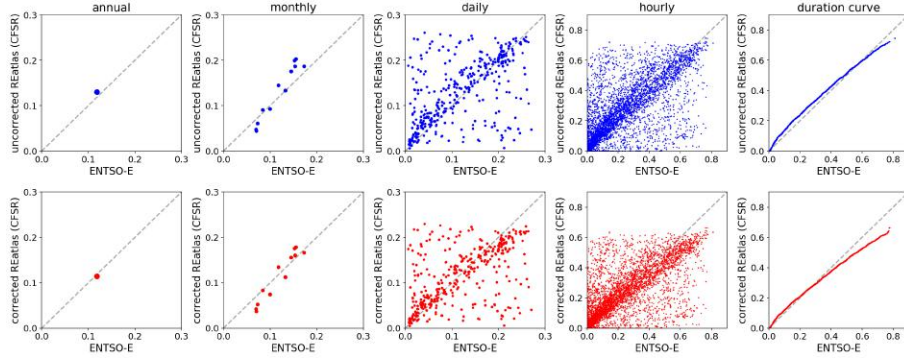

Figure 47: QQ plots comparing modeled and historical capacity factors for Czech Republic integrated throughout four different time periods (from left to right: year, month, day, hour). The rightest column shows the QQ plot for the duration curve (sorted hourly capacity factors).

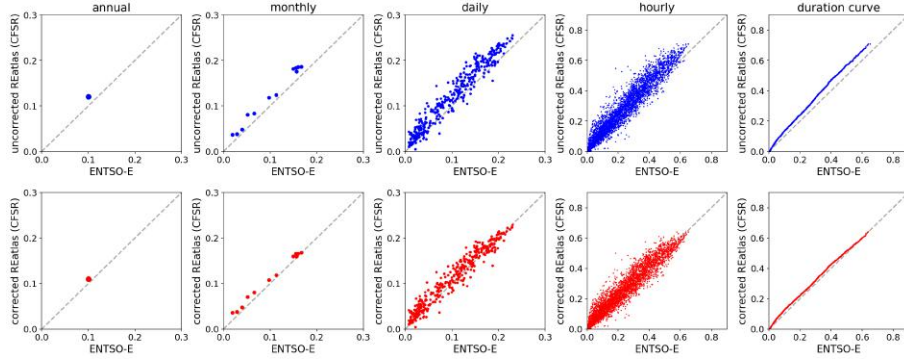

Figure 48: QQ plots comparing modeled and historical capacity factors for Germany integrated throughout four different time periods (from left to right: year, month, day, hour). The rightest column shows the QQ plot for the duration curve (sorted hourly capacity factors).

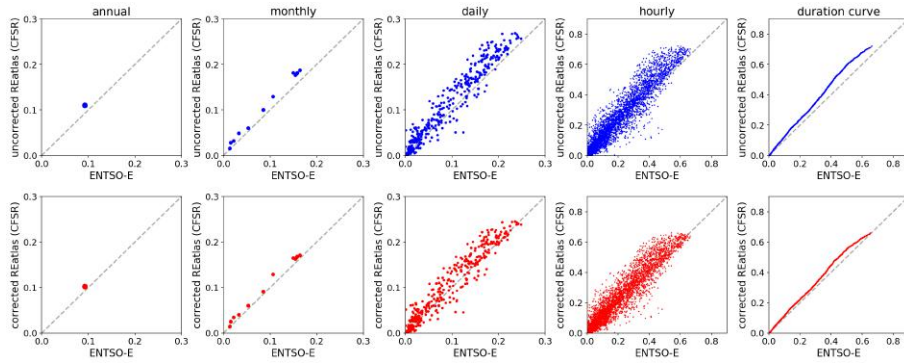

Figure 49: QQ plots comparing modeled and historical capacity factors for Denmark integrated throughout four different time periods (from left to right: year, month, day, hour). The rightest column shows the QQ plot for the duration curve (sorted hourly capacity factors).



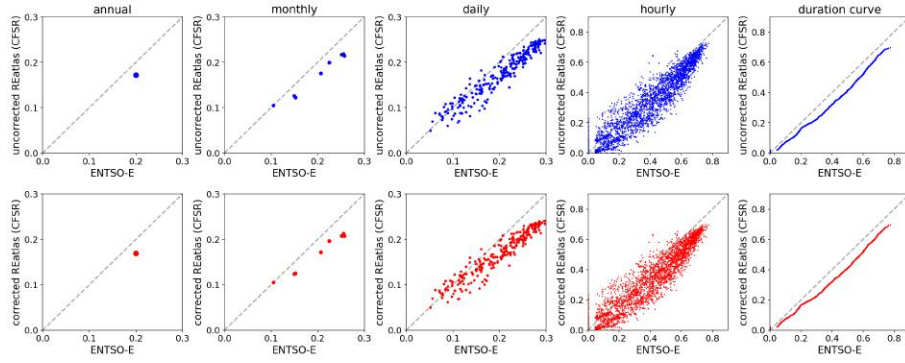

Figure 50: QQ plots comparing modeled and historical capacity factors for Spain integrated throughout four different time periods (from left to right: year, month, day, hour). The rightest column shows the QQ plot for the duration curve (sorted hourly capacity factors).

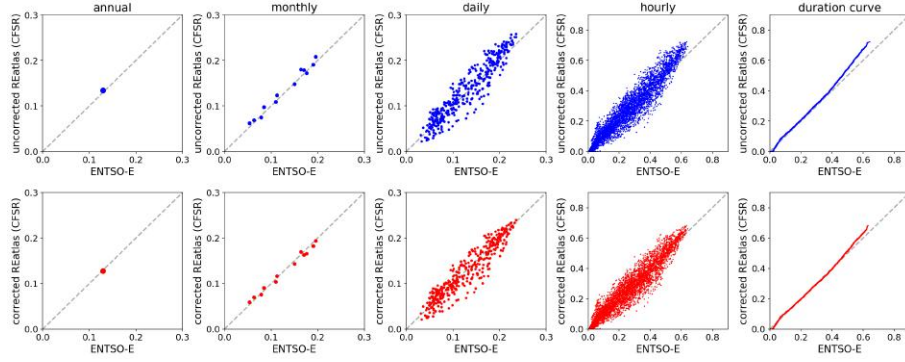

Figure 51: QQ plots comparing modeled and historical capacity factors for France integrated throughout four different time periods (from left to right: year, month, day, hour). The rightest column shows the QQ plot for the duration curve (sorted hourly capacity factors).

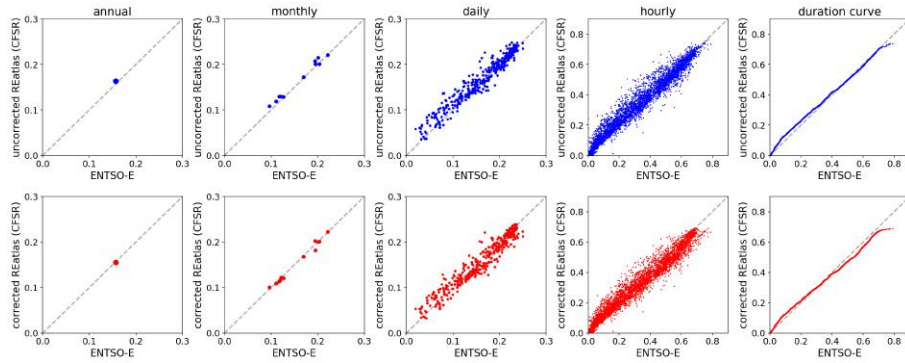

Figure 52: QQ plots comparing modeled and historical capacity factors for Greece integrated throughout four different time periods (from left to right: year, month, day, hour). The rightest column shows the QQ plot for the duration curve (sorted hourly capacity factors).

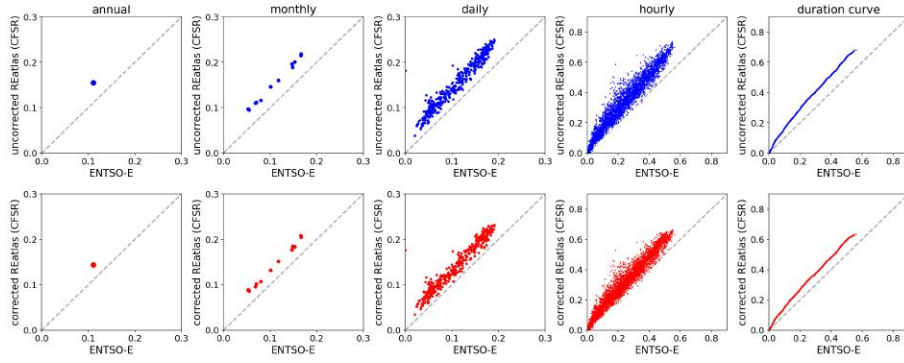

Figure 53: QQ plots comparing modeled and historical capacity factors for Italy integrated throughout four different time periods (from left to right: year, month, day, hour). The rightest column shows the QQ plot for the duration curve (sorted hourly capacity factors).

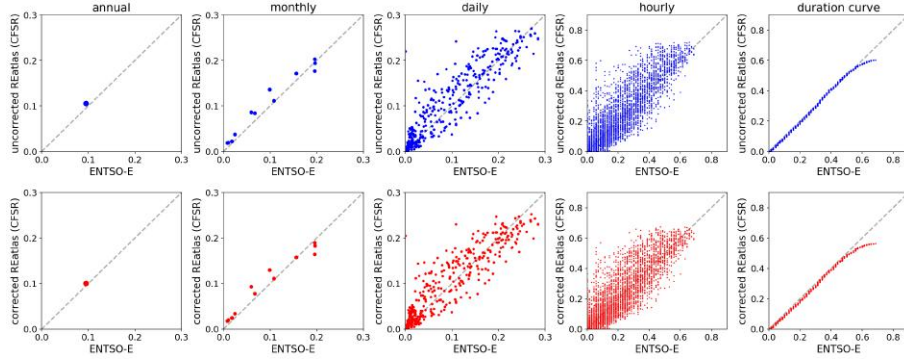

Figure 54: QQ plots comparing modeled and historical capacity factors for Lithuania integrated throughout four different time periods (from left to right: year, month, day, hour). The rightest column shows the QQ plot for the duration curve (sorted hourly capacity factors).

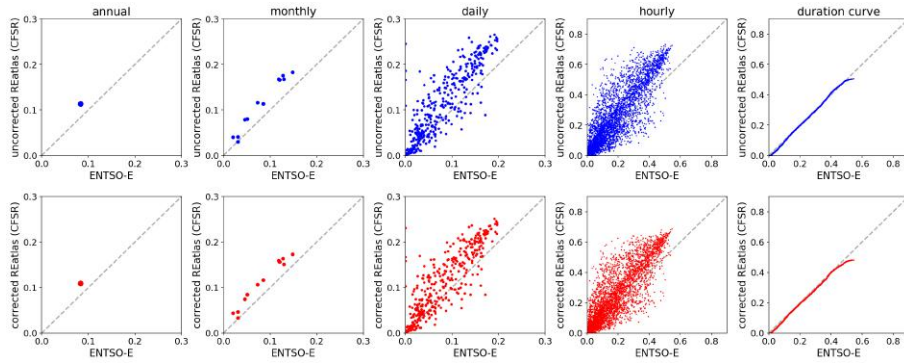

Figure 55: QQ plots comparing modeled and historical capacity factors for Netherlands integrated throughout four different time periods (from left to right: year, month, day, hour). The rightest column shows the QQ plot for the duration curve (sorted hourly capacity factors).

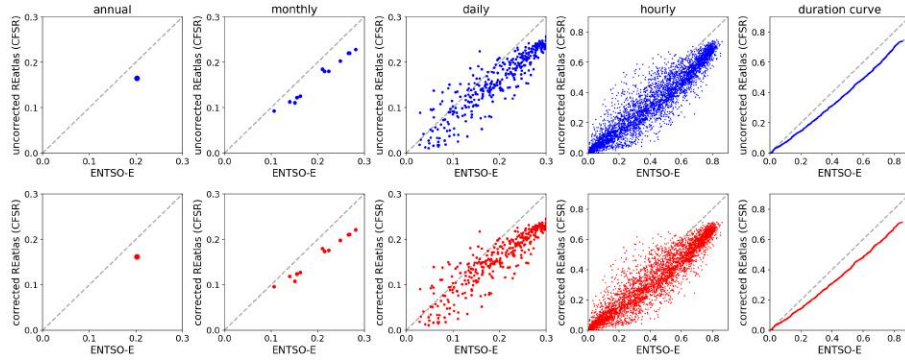

Figure 56: QQ plots comparing modeled and historical capacity factors for Portugal integrated throughout four different time periods (from left to right: year, month, day, hour). The rightest column shows the QQ plot for the duration curve (sorted hourly capacity factors).

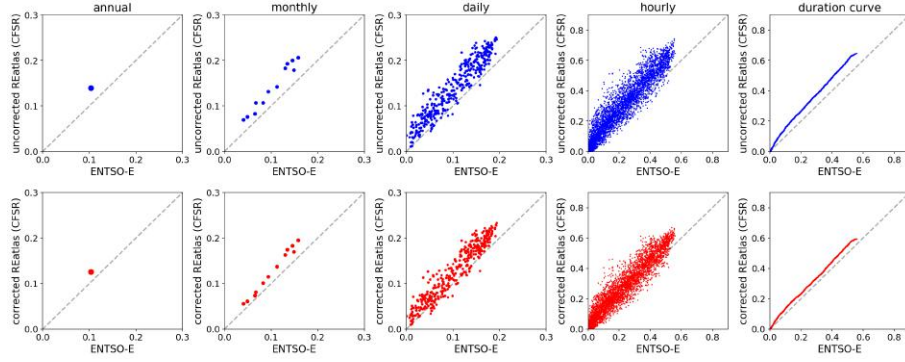

Figure 57: QQ plots comparing modeled and historical capacity factors for Romania integrated throughout four different time periods (from left to right: year, month, day, hour). The rightest column shows the QQ plot for the duration curve (sorted hourly capacity factors).

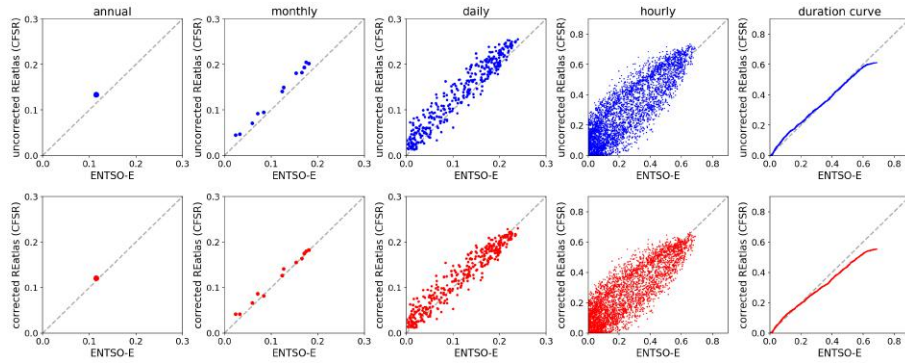

Figure 58: QQ plots comparing modeled and historical capacity factors for Slovakia integrated throughout four different time periods (from left to right: year, month, day, hour). The rightest column shows the QQ plot for the duration curve (sorted hourly capacity factors).

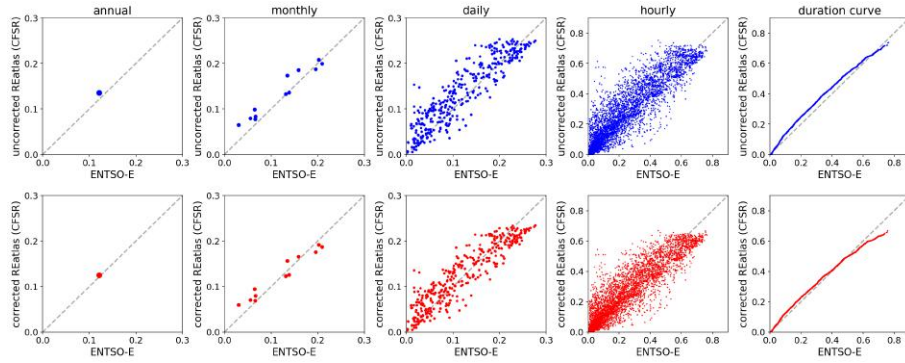

Figure 59: QQ plots comparing modeled and historical capacity factors for Slovenia integrated throughout four different time periods (from left to right: year, month, day, hour). The rightest column shows the QQ plot for the duration curve (sorted hourly capacity factors).

## 5. Global modeled and historical time series comparison

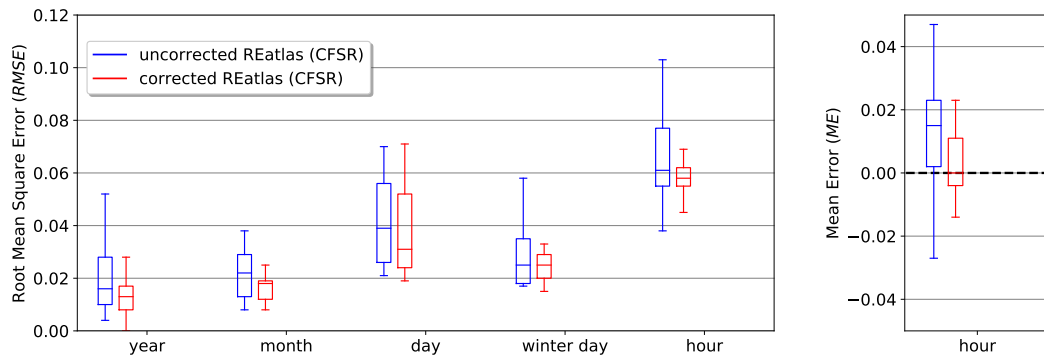

Figure 60: (left) Root Mean Square Error ( $RMSE$ ) and Mean Error ( $ME$ ) calculated comparing simulated and historical time series for 2016 and 15 countries.

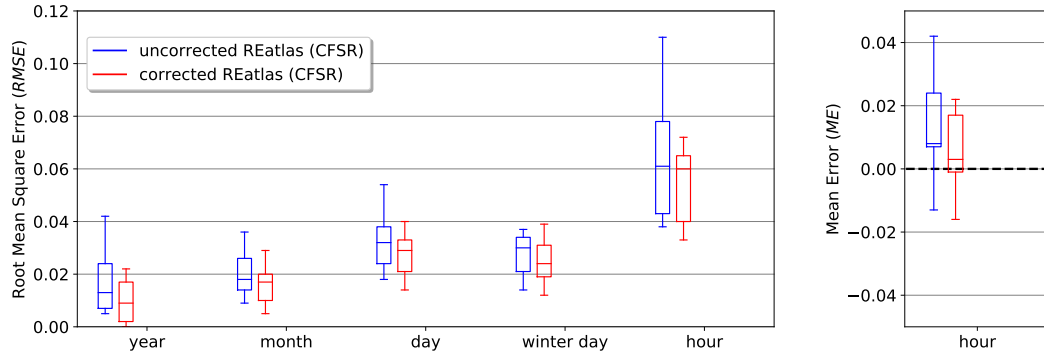

Figure 61: (left) Root Mean Square Error ( $RMSE$ ) and Mean Error ( $ME$ ) calculated comparing simulated and historical time series for 2017 and 15 countries.

## 6. Ramps

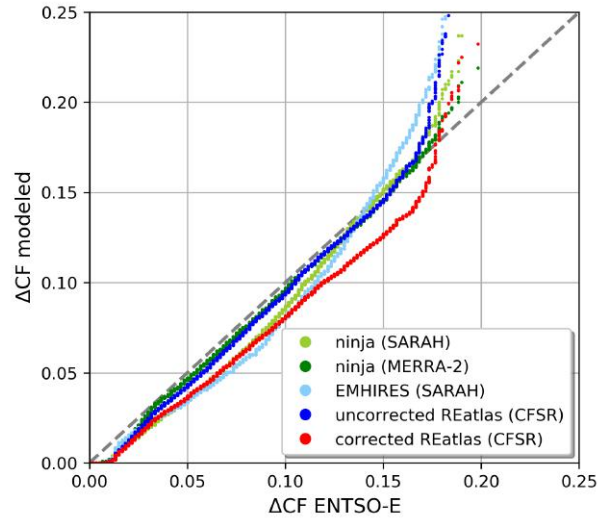

Figure 62: QQ plot for the duration curve of the ramps  $\Delta CF$  in Austria .

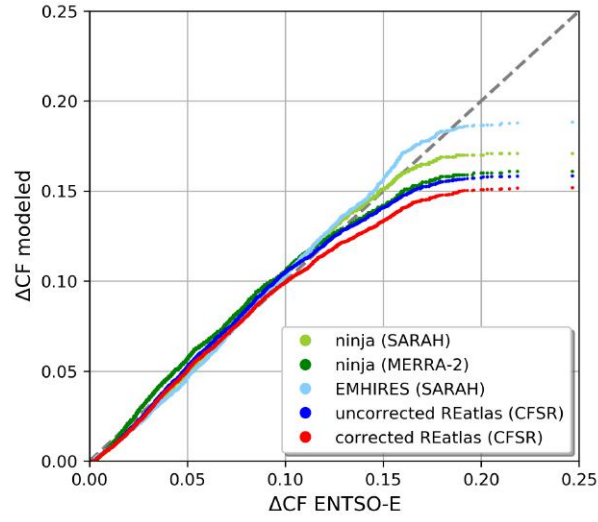

Figure 63: QQ plot for the duration curve of the ramps  $\Delta CF$  in Belgium .

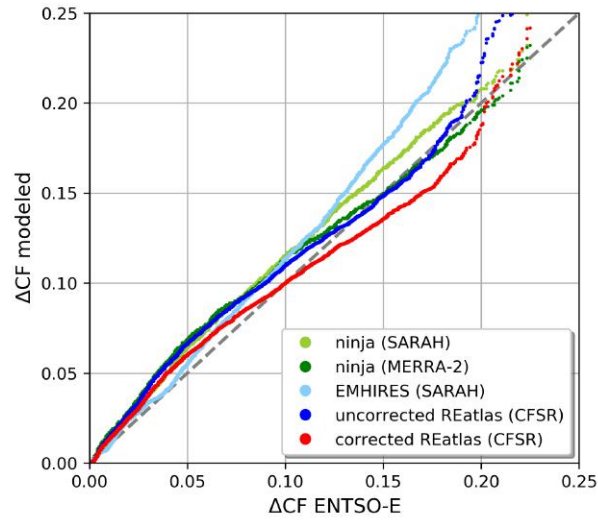

Figure 64: QQ plot for the duration curve of the ramps  $\Delta CF$  in Bulgaria .

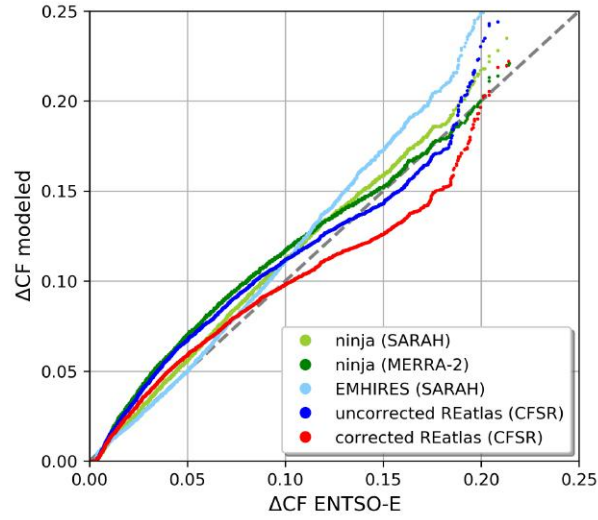

Figure 65: QQ plot for the duration curve of the ramps  $\Delta CF$  in Czech Republic .

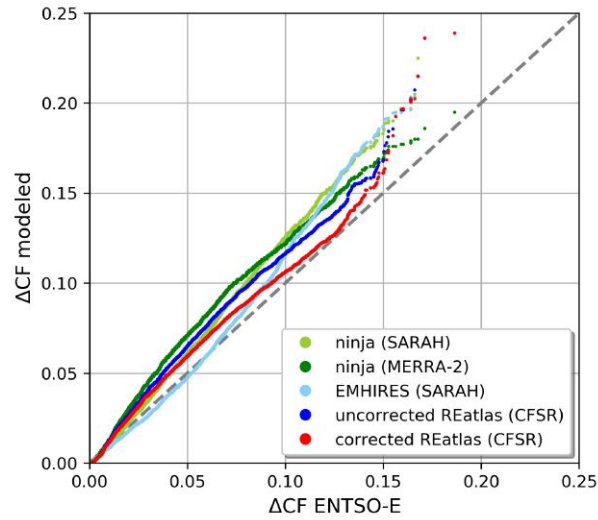

Figure 66: QQ plot for the duration curve of the ramps  $\Delta CF$  in Germany .



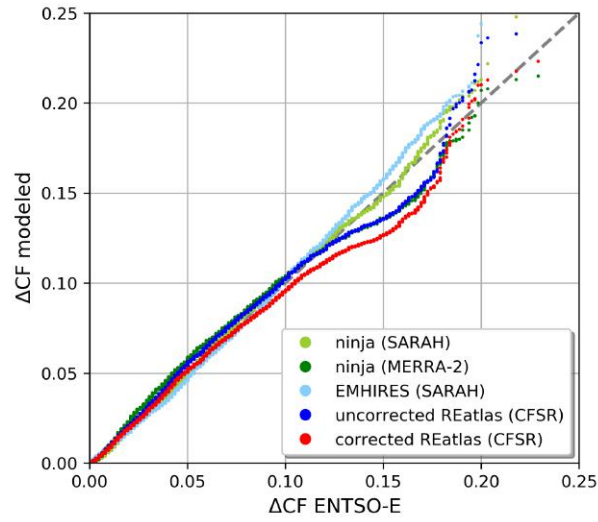

Figure 67: QQ plot for the duration curve of the ramps  $\Delta CF$  in Denmark .

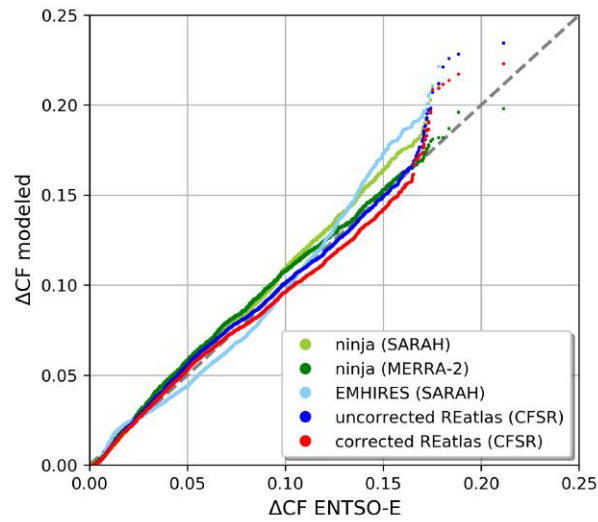

Figure 68: QQ plot for the duration curve of the ramps  $\Delta CF$  in France .



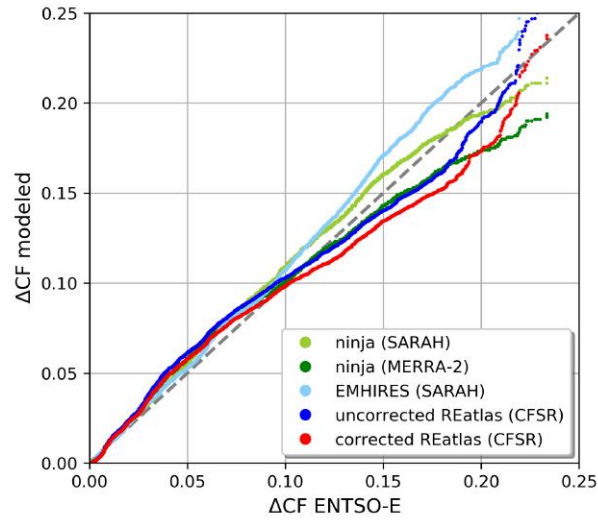

Figure 69: QQ plot for the duration curve of the ramps  $\Delta CF$  in Greece .

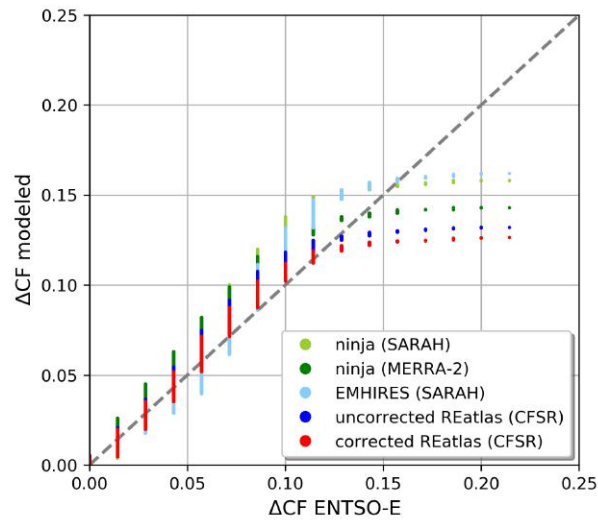

Figure 70: QQ plot for the duration curve of the ramps  $\Delta CF$  in Lithuania .

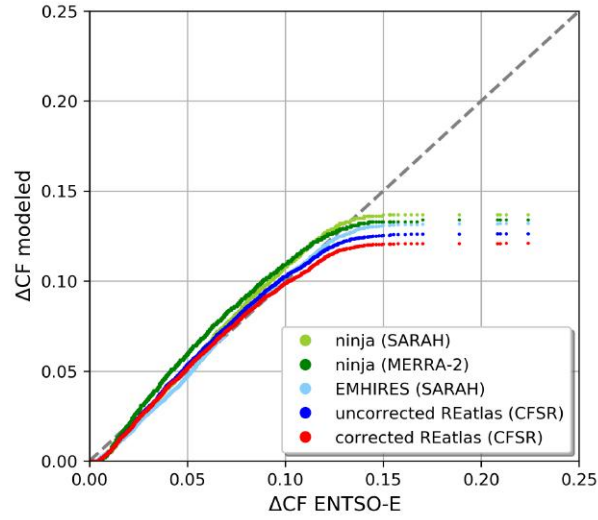

Figure 71: QQ plot for the duration curve of the ramps  $\Delta CF$  in Netherlands .

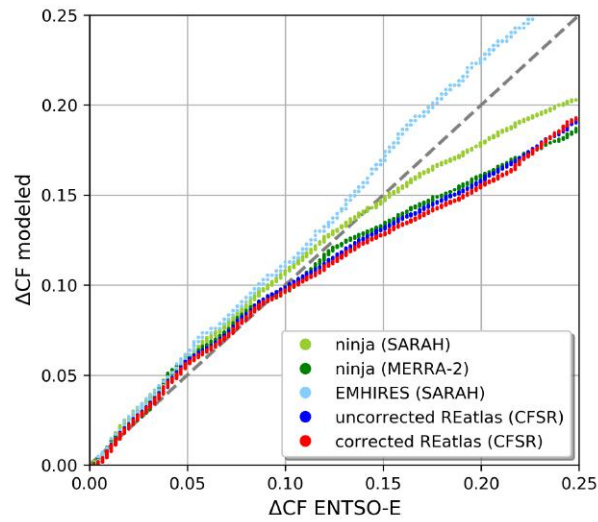

Figure 72: QQ plot for the duration curve of the ramps  $\Delta CF$  in Portugal .

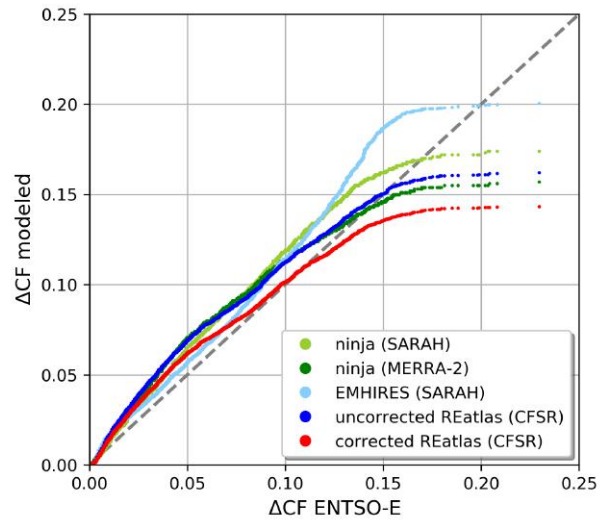

Figure 73: QQ plot for the duration curve of the ramps  $\Delta CF$  in Romania .

## 7. Impact of the PV system configuration on the mismatch curves

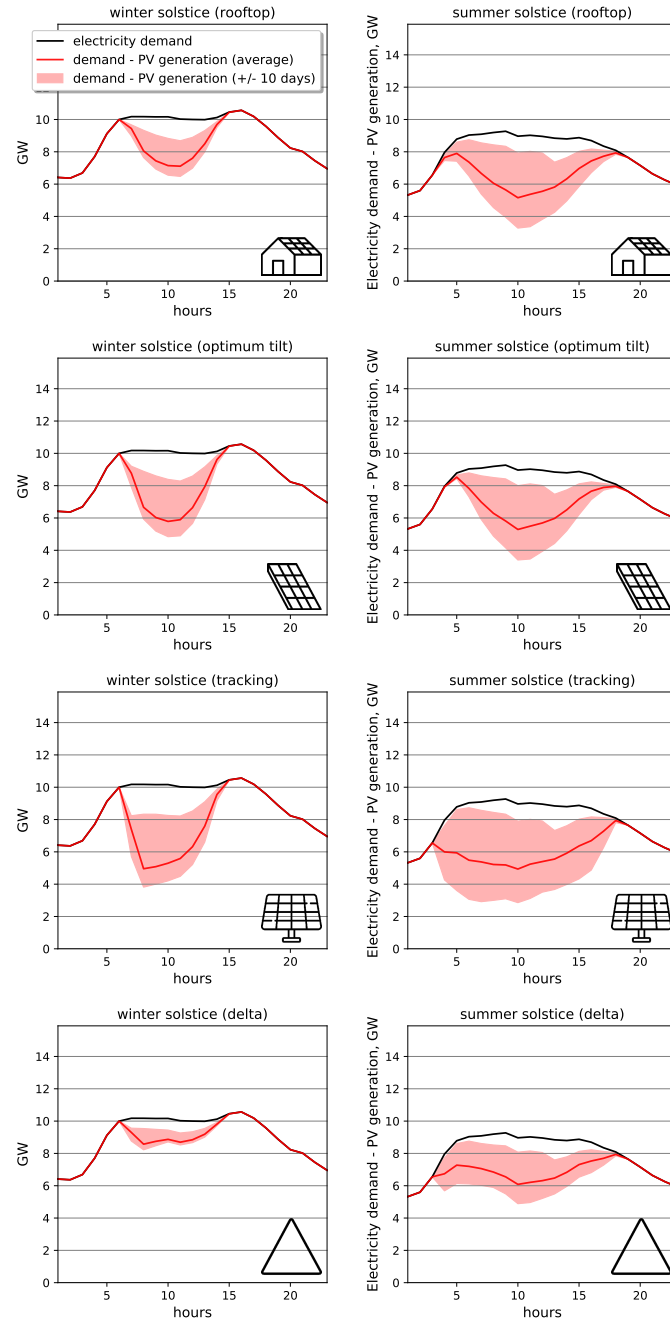

Figure 74: Electricity demand minus PV generation for winter and summer solstice in Austria , assuming different configurations for the PV panels in the country.

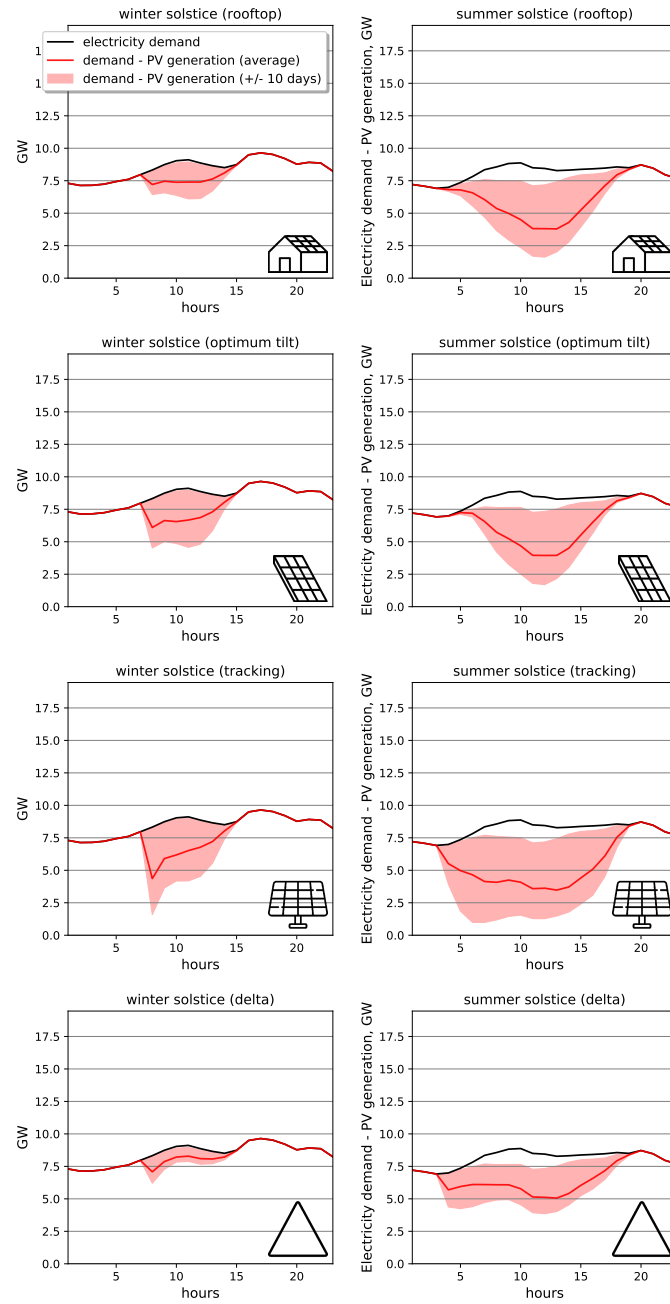

Figure 75: Electricity demand minus PV generation for winter and summer solstice in Belgium , assuming different configurations for the PV panels in the country.

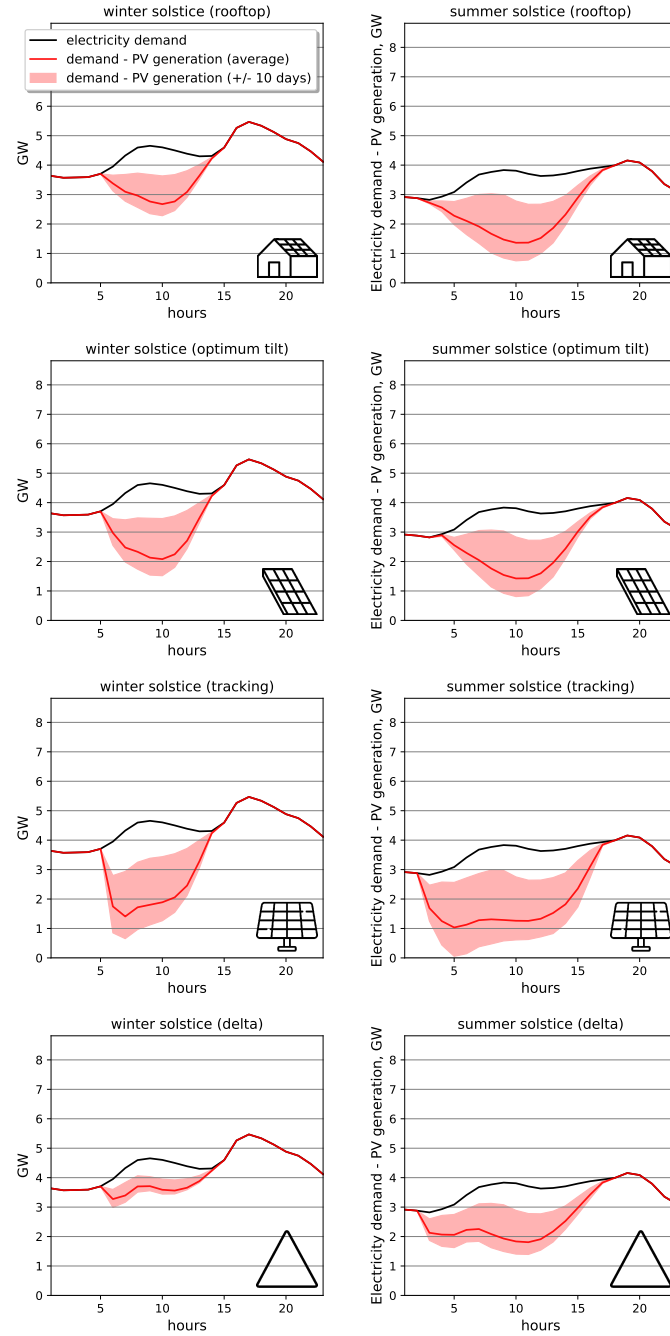

Figure 76: Electricity demand minus PV generation for winter and summer solstice in Bulgaria , assuming different configurations for the PV panels in the country.

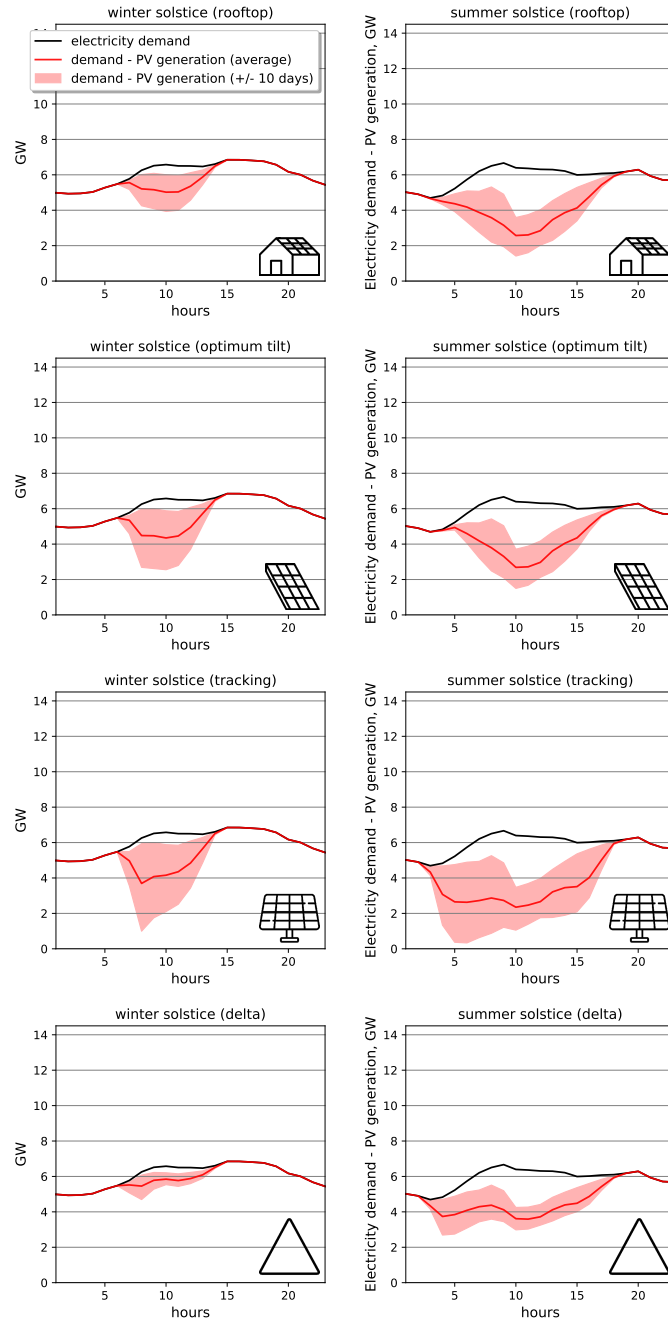

Figure 77: Electricity demand minus PV generation for winter and summer solstice in Czech Republic , assuming different configurations for the PV panels in the country.

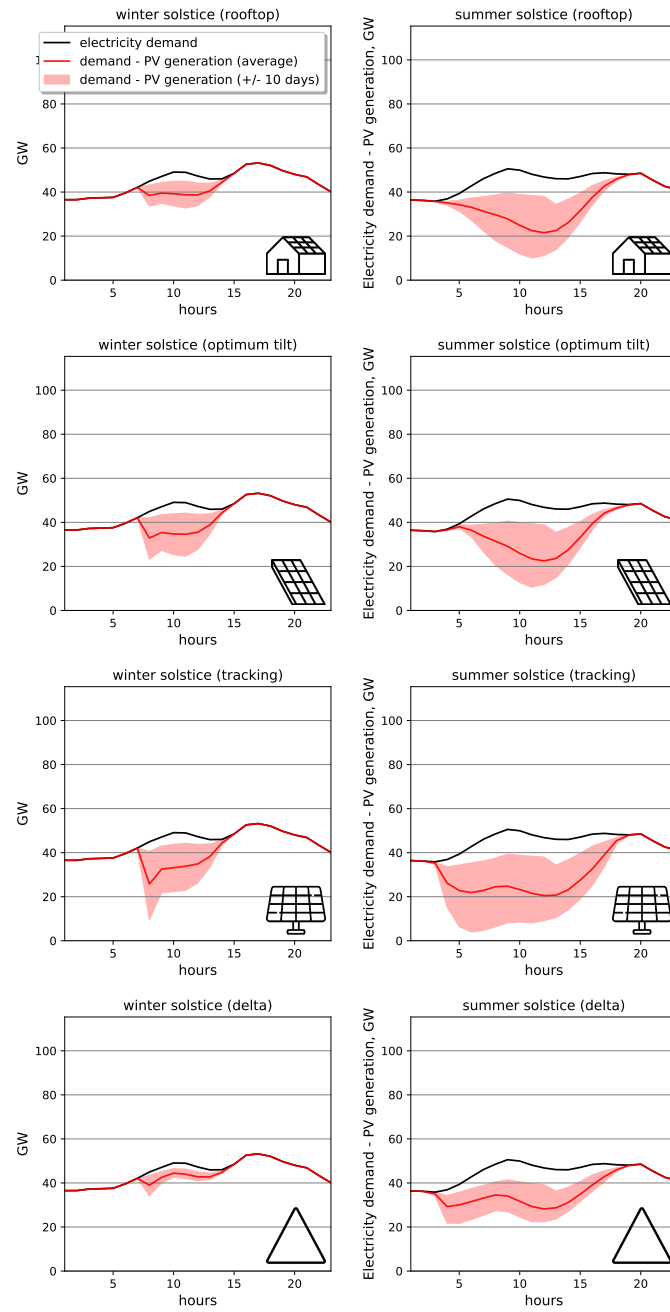

Figure 78: Electricity demand minus PV generation for winter and summer solstice in Germany , assuming different configurations for the PV panels in the country.



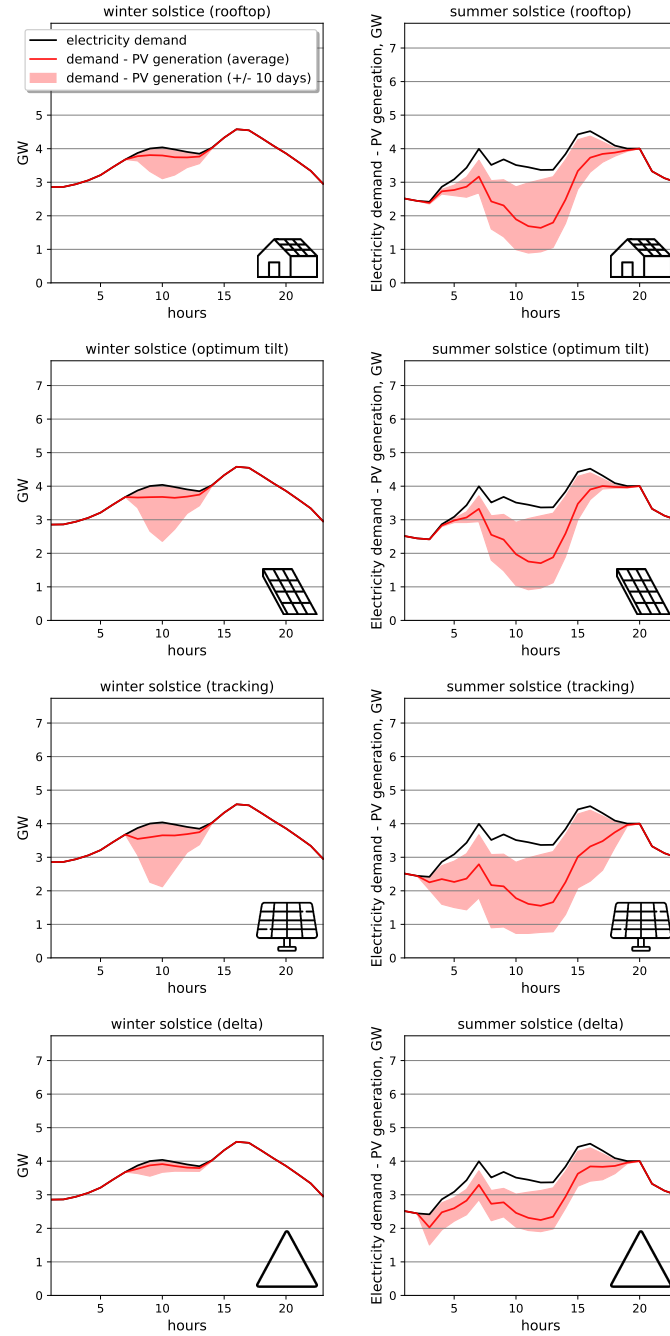

Figure 79: Electricity demand minus PV generation for winter and summer solstice in Denmark , assuming different configurations for the PV panels in the country.

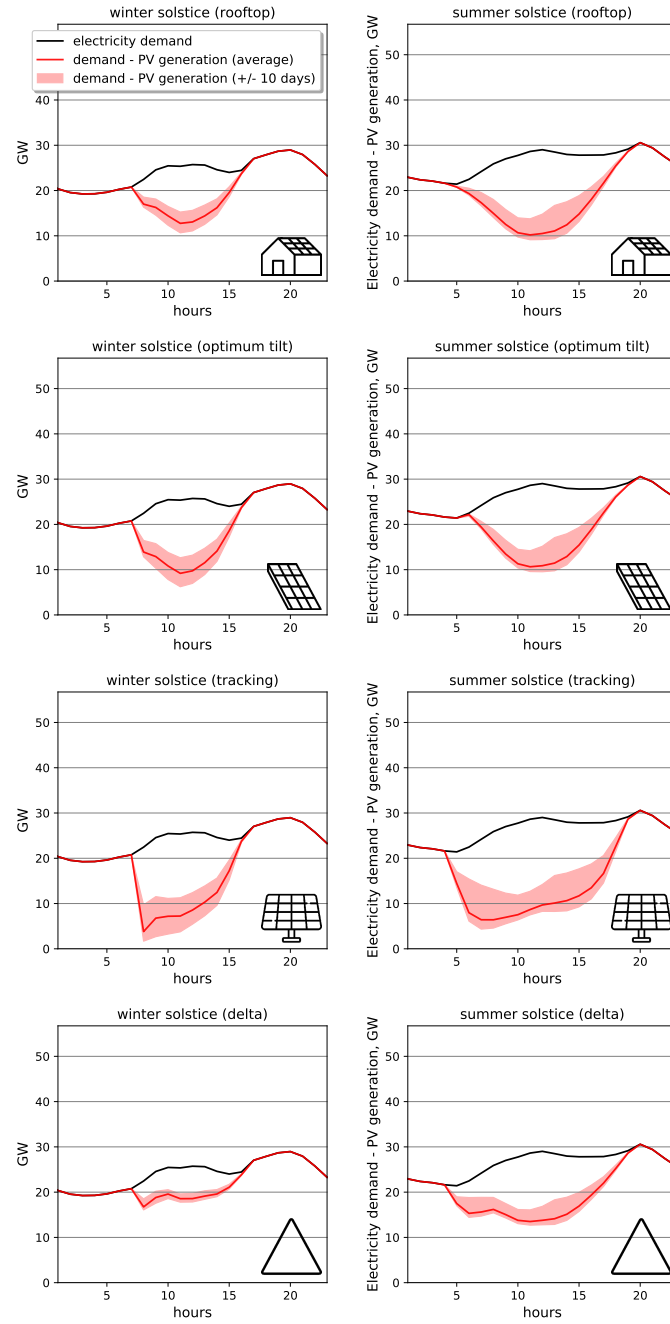

Figure 80: Electricity demand minus PV generation for winter and summer solstice in Spain , assuming different configurations for the PV panels in the country.

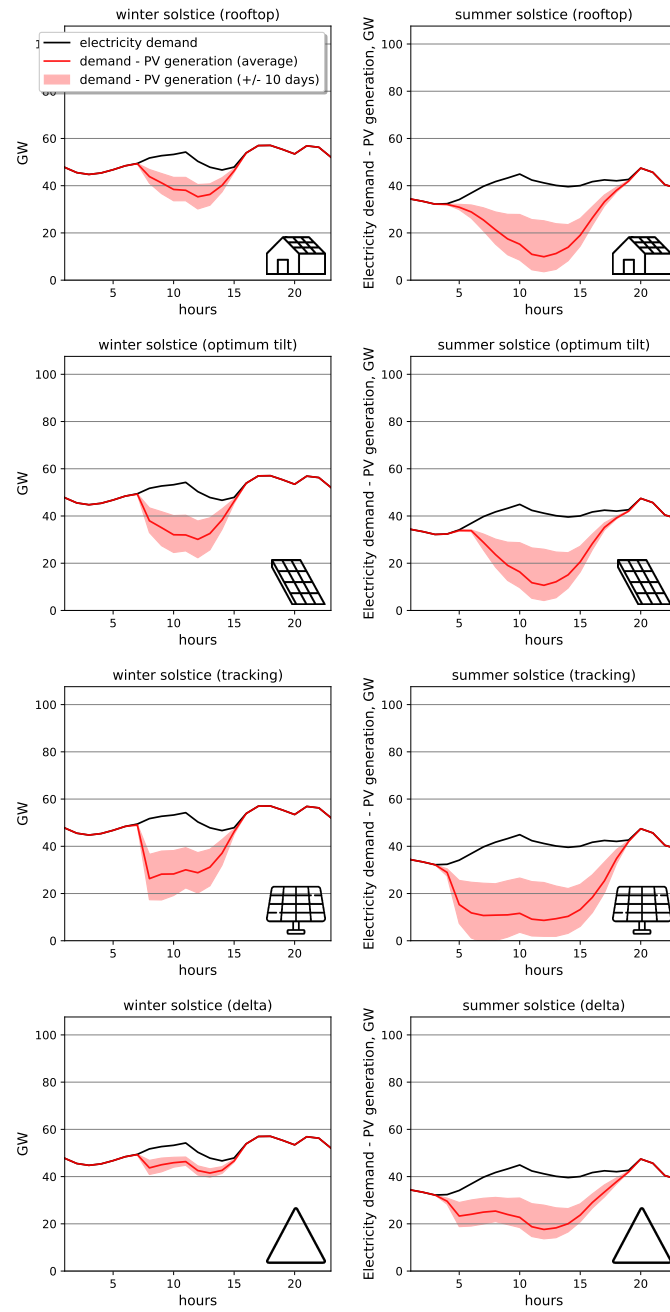

Figure 81: Electricity demand minus PV generation for winter and summer solstice in France , assuming different configurations for the PV panels in the country.

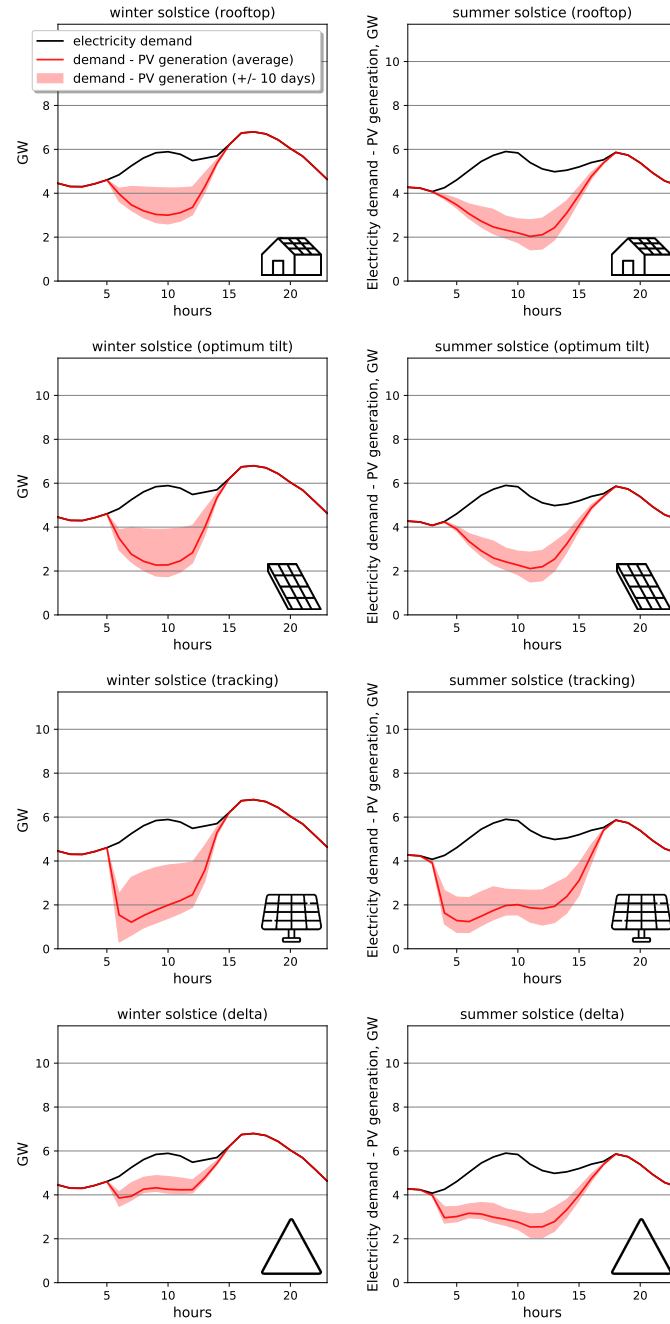

Figure 82: Electricity demand minus PV generation for winter and summer solstice in Greece , assuming different configurations for the PV panels in the country.

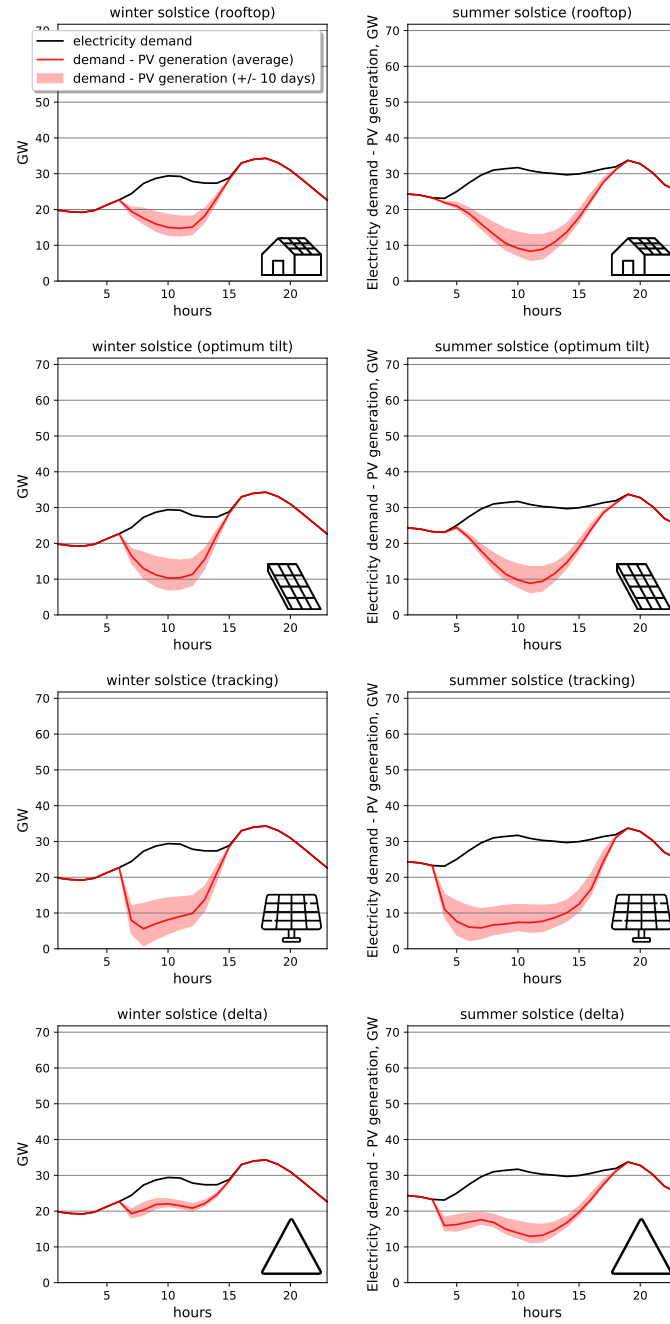

Figure 83: Electricity demand minus PV generation for winter and summer solstice in Italy , assuming different configurations for the PV panels in the country.

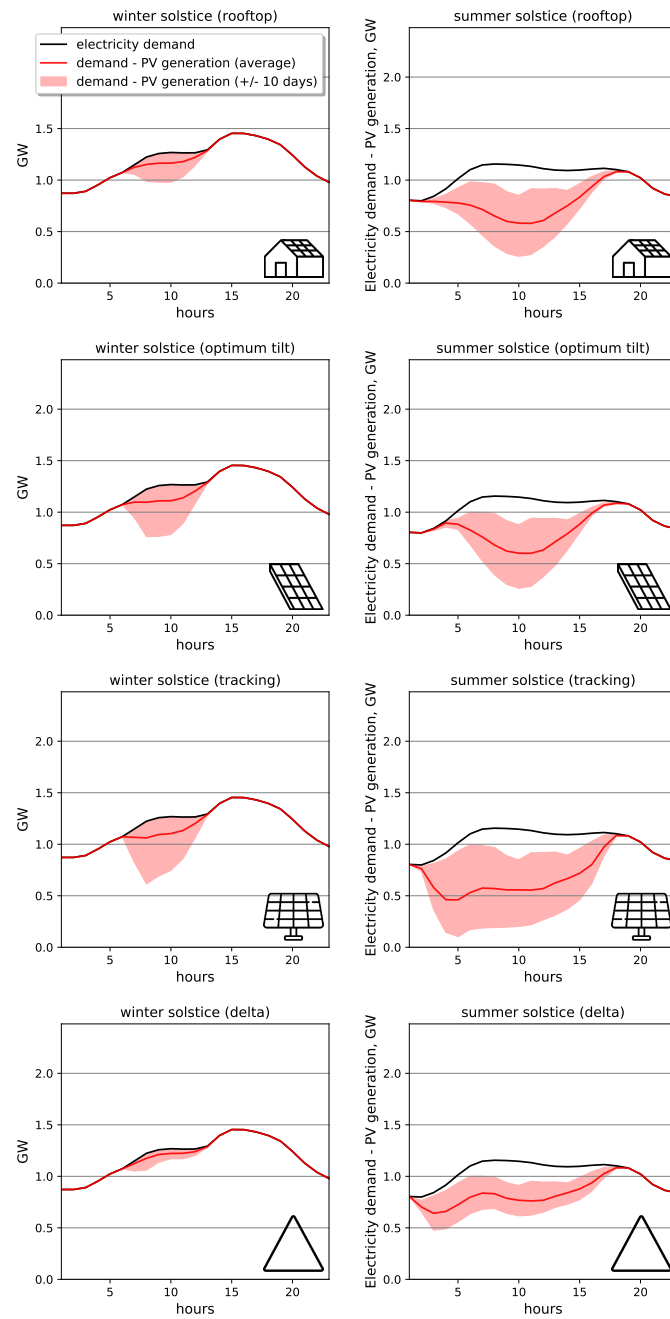

Figure 84: Electricity demand minus PV generation for winter and summer solstice in Lithuania , assuming different configurations for the PV panels in the country.

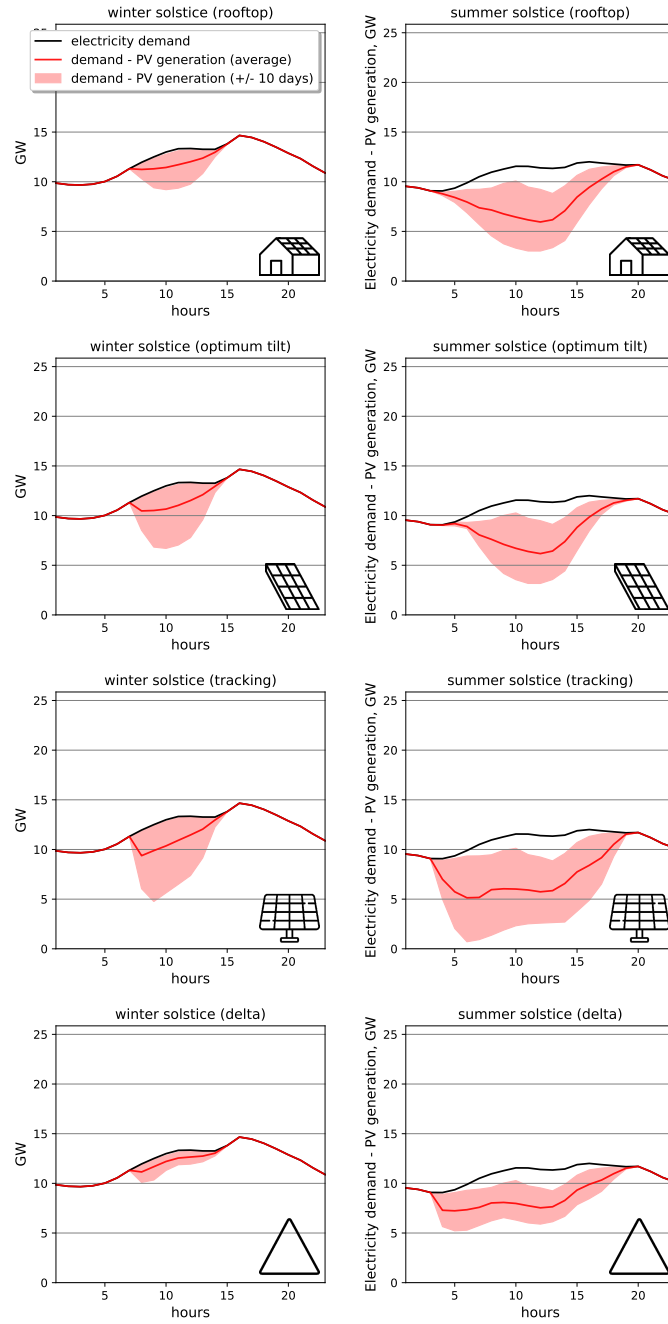

Figure 85: Electricity demand minus PV generation for winter and summer solstice in Netherlands , assuming different configurations for the PV panels in the country.

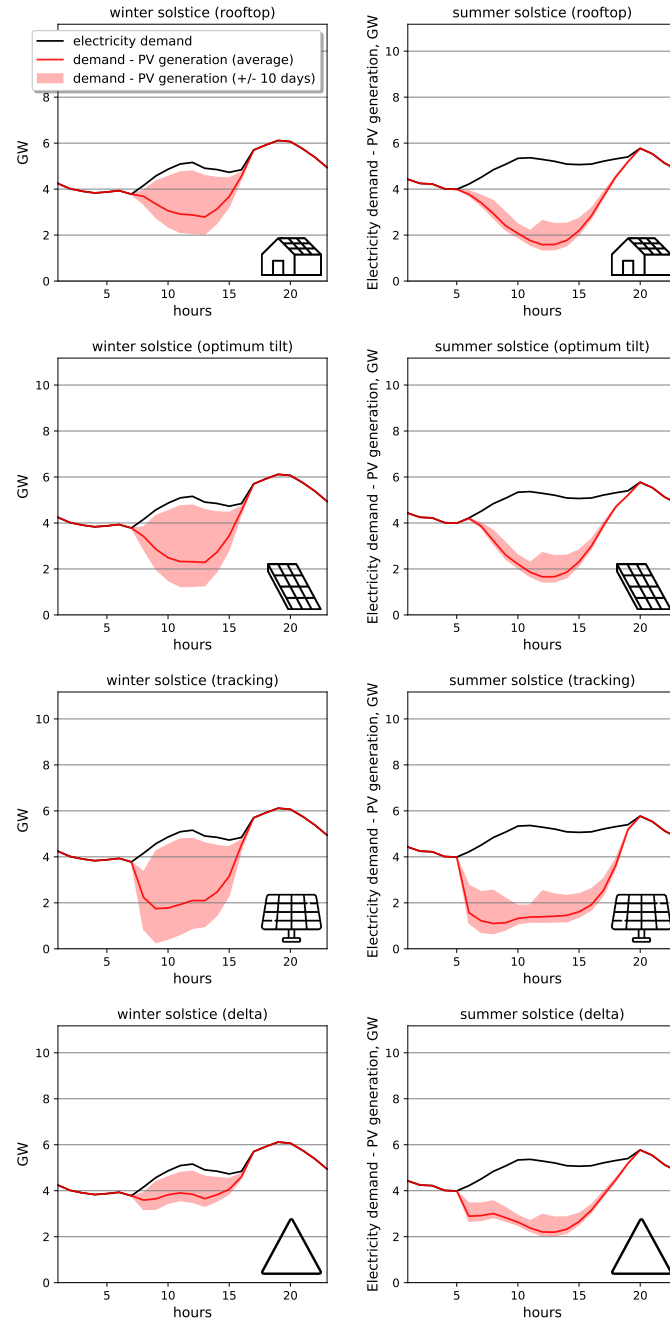

Figure 86: Electricity demand minus PV generation for winter and summer solstice in Portugal , assuming different configurations for the PV panels in the country.



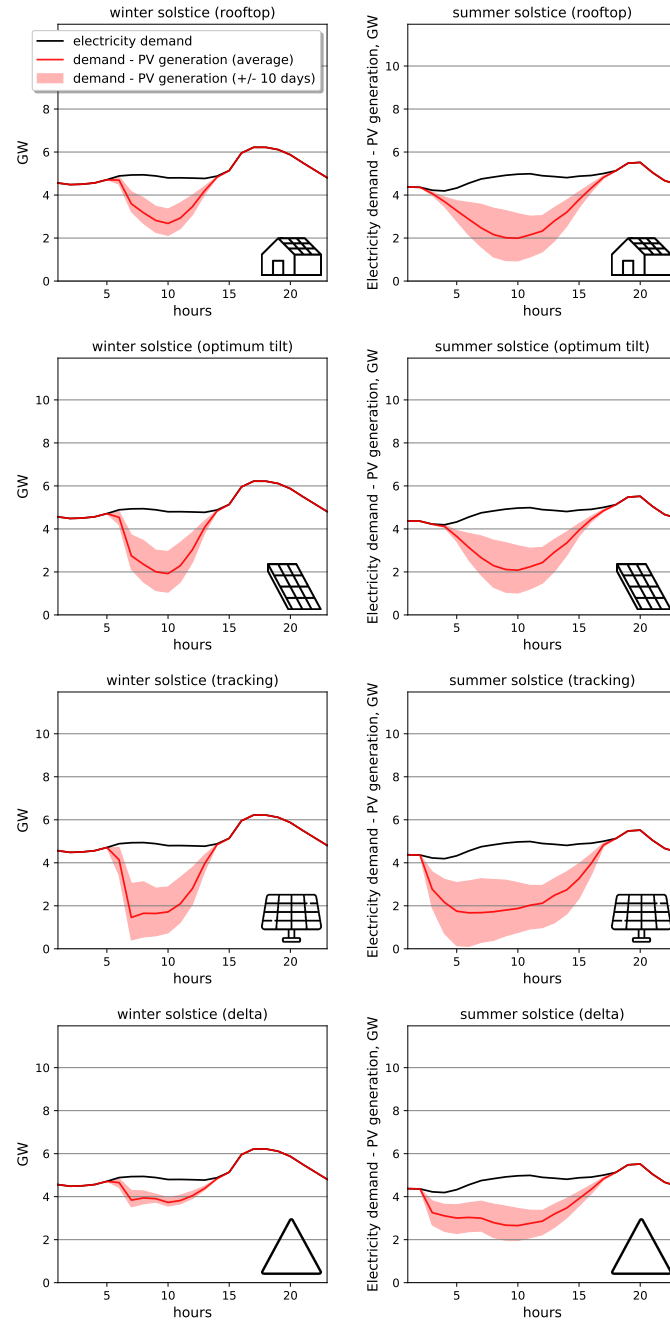

Figure 87: Electricity demand minus PV generation for winter and summer solstice in Romania , assuming different configurations for the PV panels in the country.

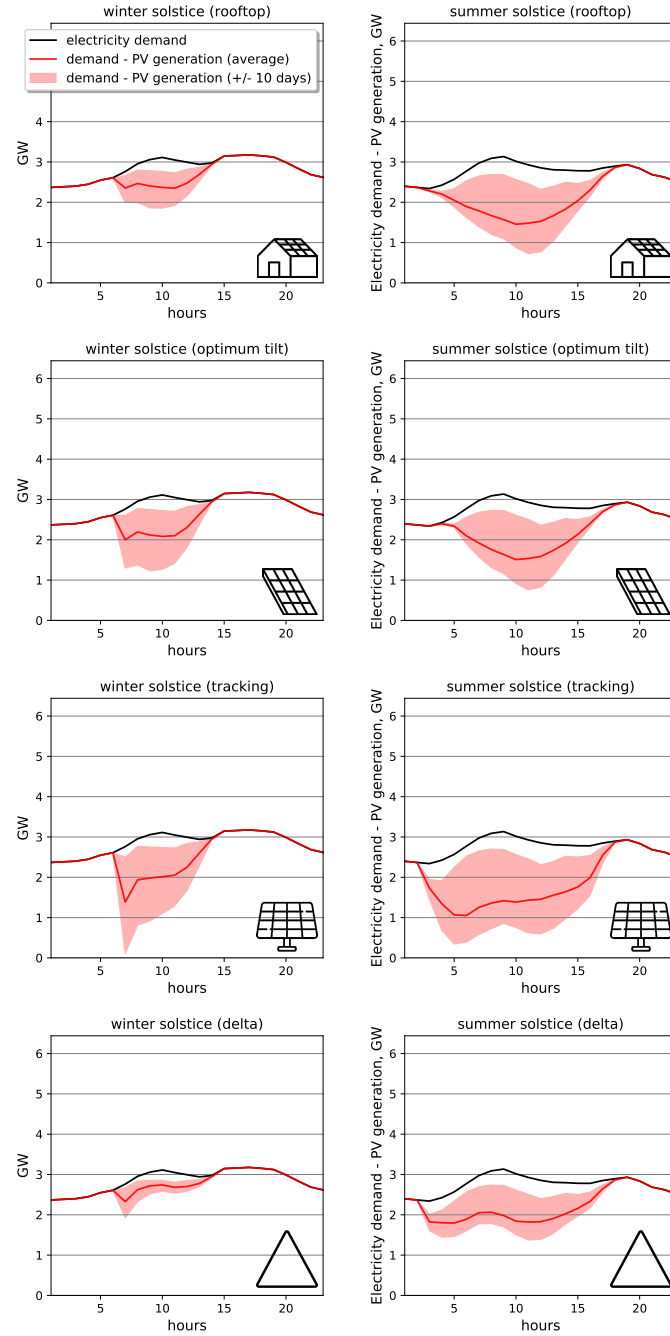

Figure 88: Electricity demand minus PV generation for winter and summer solstice in Slovakia , assuming different configurations for the PV panels in the country.

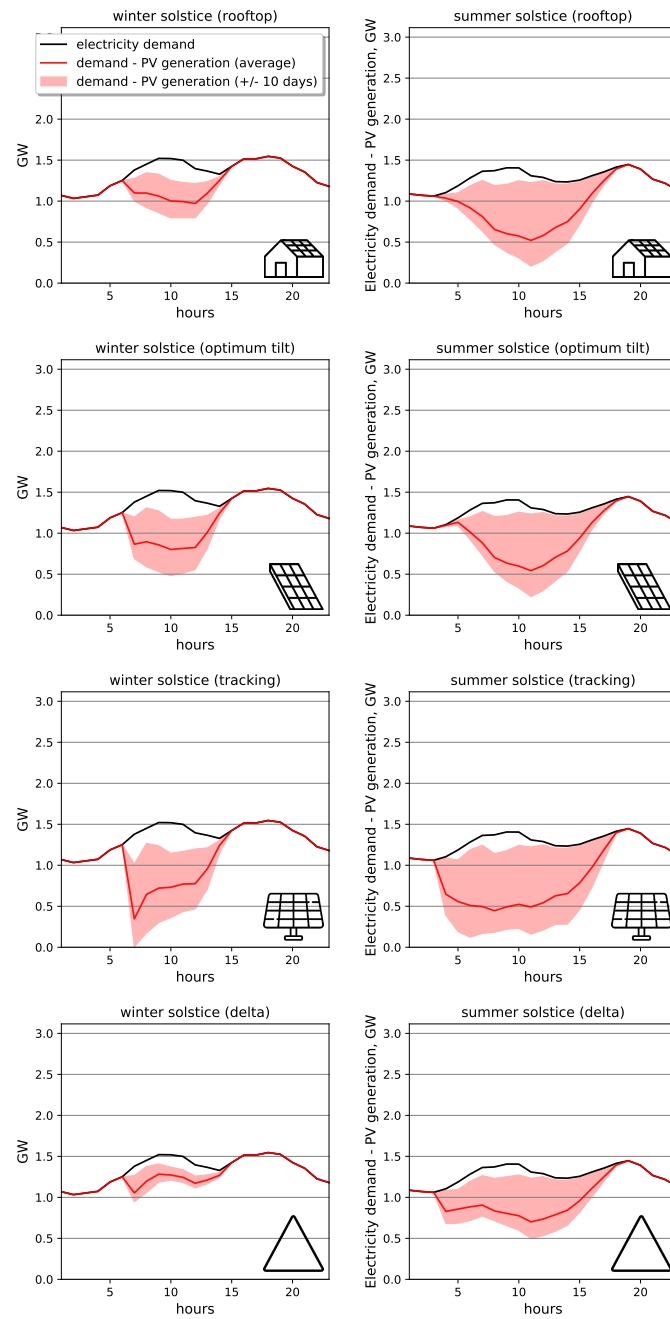

Figure 89: Electricity demand minus PV generation for winter and summer solstice in Slovenia , assuming different configurations for the PV panels in the country.
